# Supplementary material for: On the Robustness of Human Pose Estimation
Source: arXiv:1908.06401 source file (2021-06-10)
Supplement: Supplementary file 1 [file supp.tex]

{\centering{\textbf {\large Appendix}}}
\appendix
\section{Experimental Details}
\label{exp_details}

\subsection{Datasets}
\noindent We first explain the two datasets - MPII\cite{andriluka14cvpr} and COCO\cite{coco} that we use to benchmark HPE models. 
\\
\\
\textbf{MPII Dataset.} It is the primary dataset for single person 2D pose estimation. The images were collected from YouTube videos, covering daily human activities with complex poses and image appearances. There are about 25k images for training set, 3k image for validation and 7k images for testing. Since we do not have annotations for the test dataset we used our validation dataset to evaluate the effectiveness of all our attacks. The metric used for this dataset is the PCKh.
\\
\\
\textbf{COCO Dataset.} The COCO Keypoint Challenge requires “in the wild” multi-person detection and pose estimation in challenging, uncontrolled conditions. The COCO train, validation, and test sets, containing more than 200k images and 250k person instances labeled with keypoints. 150k instances of them are publicly available for training and validation. The COCO evaluation defines the object keypoint similarity (OKS) and uses the mean average precision (AP) over 10 OKS thresholds as primary metric. The OKS plays the same role as IoU does in object detection. It is calculated as the distance between predicted points and ground truth points normalized by the scale of the person. Since OKS is a multiperson and a detection metric we have used PCK as our main metric for evaluation of COCO and performing adversarial attacks on COCO.

\section{Results on MPII Dataset}
In this section we provide quantitative and visual results for models trained and evaluated on the MPII dataset. We also go on to provide more details about the effect of limiting the data available for generating the adversarial perturbations on the effectiveness of the perturbations.

\subsection {Detailed Results}

\par In this section we evaluate all the models when subjected to each adversarial attack. The values in Tables \ref{table:UI_20} and \ref{table:UF} represent the relative PCKh on the validation set while those in Tables \ref{table:TI_20} and \ref{table:TF} represent the target PCKh with respect to the new target. Table \ref{table:originalPerformance} lists the PCKh of the different model on the validation set under our experimental set up. Since we do not use multiple crops, flipping and other methods to provide further boosts in performance, the numbers we report are slightly inferior to the ones originally reported in the relevant papers in some cases.

\subsection{Results with 100 iterations} \label{hundrediter}
We also perform the iterative attacks for 100 iterations and compare the different model in Fig.  \ref{fig:IGSM_100}. On increasing the number of iterations and $epsilon$, performance of all models falls to zero in untargeted attacks and approaches nineties in targeted setting, showing that given enough computational and time resources we can attack virtually every image in both a targeted and untargeted fashion.

\begin{figure*}[]
\centering
    \subfloat[Plots for performance of different models under IGSM-U-100 attacks \label{fig:ui_100}]{
        \includegraphics[width=0.4\linewidth]{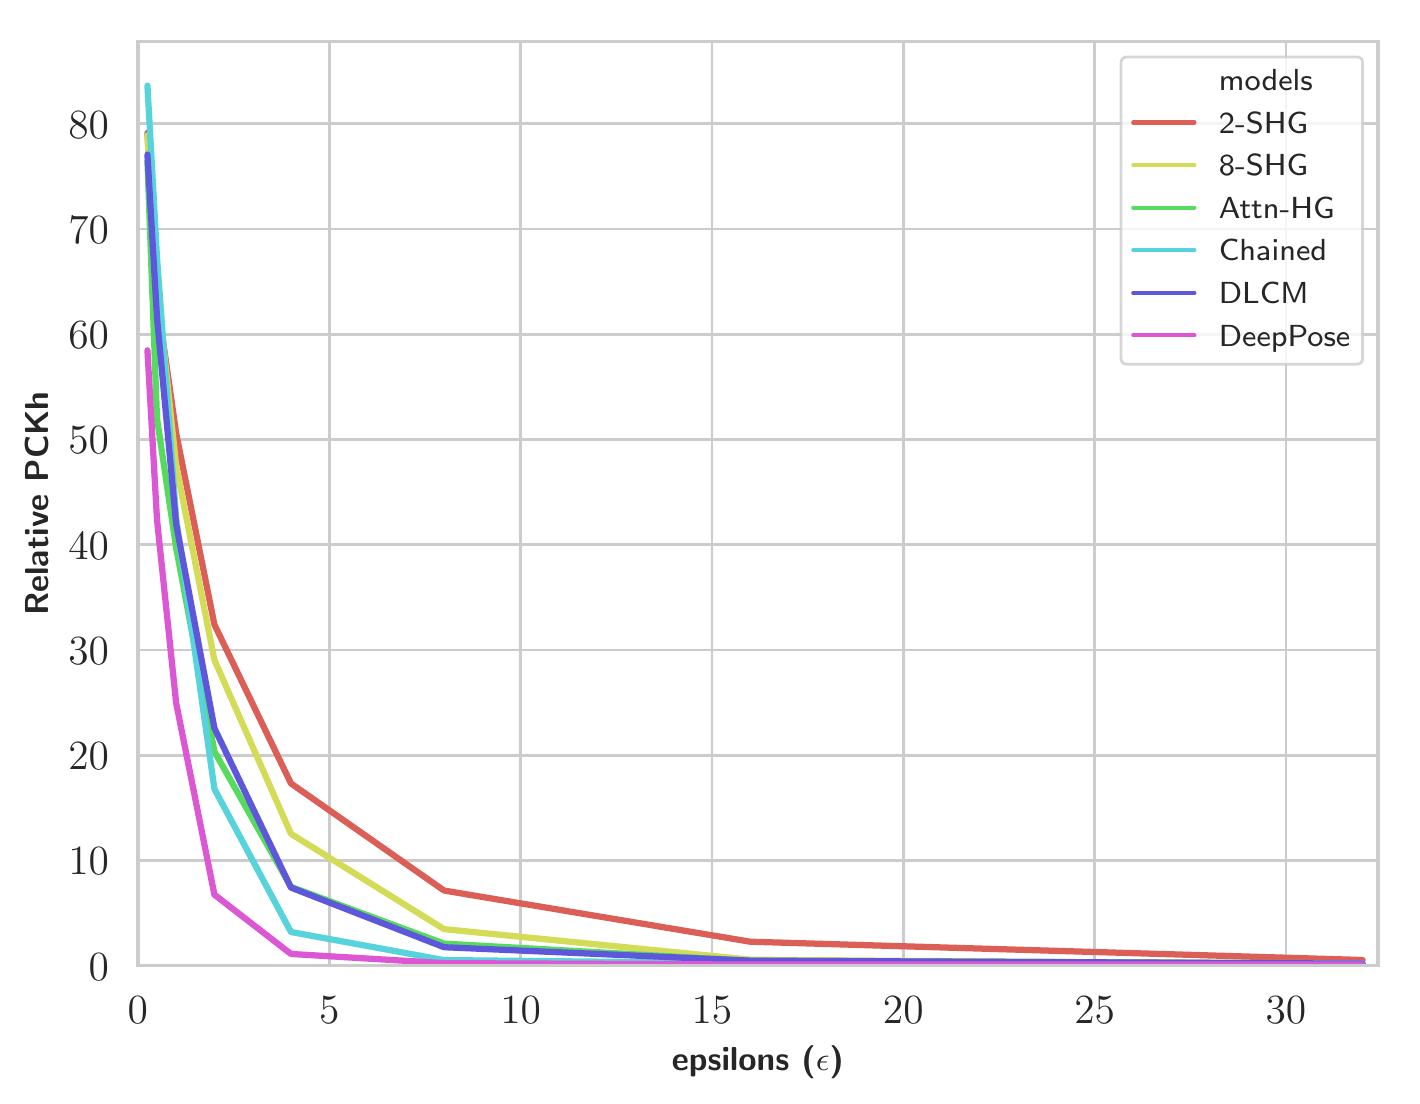}}
    \hfill
    \subfloat[Plots for performance of different models under IGSM-T-100 attacks]{
        \includegraphics[width=0.4\linewidth]{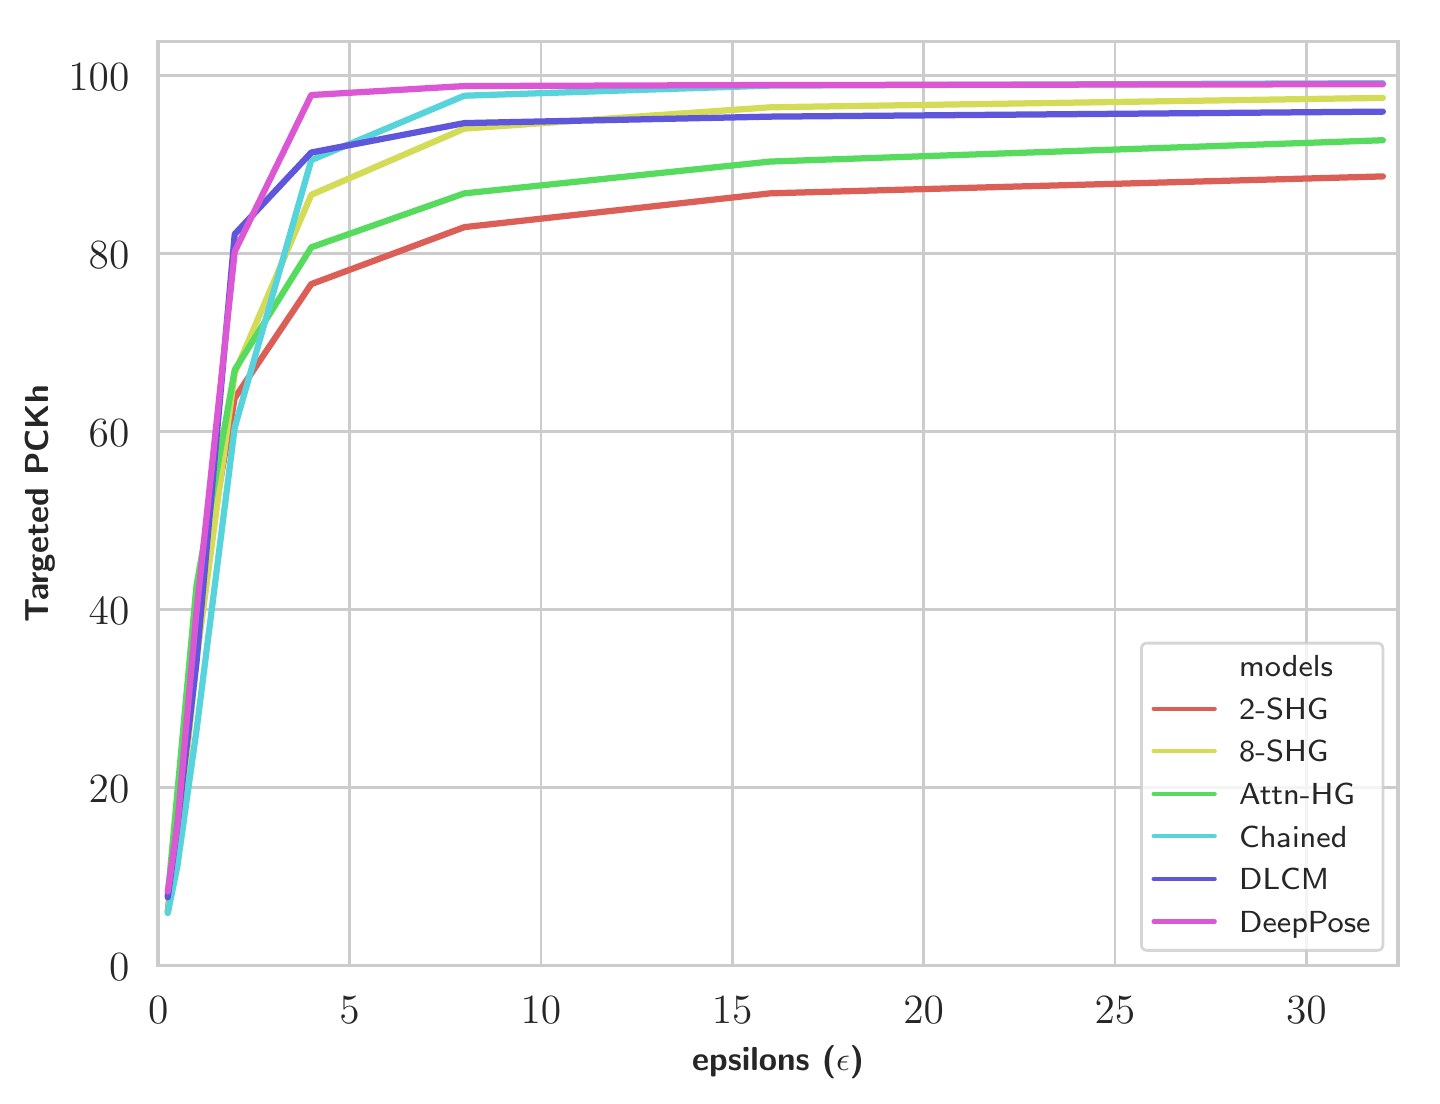}}

\caption{Untargeted and targeted iterative attacks with 100 iterations on all models}
\label{fig:IGSM_100}
\end{figure*}

\vspace{-5pt}

\subsection {Effect of Amount of Data on Universal Perturbations}
\par We demonstrate that the universal perturbations are effective attacks even on limiting the amount of data used to generate them. We limit the number of images used to generate the perturbation and then use the (previously unseen) validation set to quantify the effectiveness of the attack which shows the tremendous ability of these computationally light yet potent attacks to generalize across images. We perform this experiment on the 8-Stacked-Hourglass which forms the backbone for a lot of the other models. 

\par We also provide a visualization of the perturbations generated in each case in Fig \ref{fig:UniversalAdversarial_small}.  It is interesting to notice that as the number of samples used increases, the perturbations start to resemble humans more and more. In particular, the effectiveness increases markedly when we move from 512 to 1250 training samples, and when we compare perturbations generated using less than 512 images and more than 1250 images, we can see that the human shape (with a head and hands) starts to become discernible for the first time at 1250 images. On fewer images, the perturbation simply tries to hallucinate limbs all over the image in an attempt to fool the network.

\par We also provide a table for the doubly general universal perturbations for $\epsilon = 8$.

\section{Results on COCO Dataset}
We also discuss the results on the COCO Keypoints benchmark. COCO is mainly a multiperson keypoint detection benchmark. Note that we do not compute adversarial perturbations for any of the large 5/8 stacks models on COCO and hence only Chained, DeepPose and 2-SHG have been used. The original performance is present in Table \ref{table:COCO_original}.

\subsection{Extensive Results}
We performed all four combinations of {Targeted, Untargeted} and {Fast, Iterative} attacks on the validation set of COCO benchmarks. Tables \ref{table:COCO_UI}, \ref{table:COCO_TI}, \ref{table:COCO_UF} and \ref{table:COCO_TF} show the results on all combinations of these attacks.

\subsection{Evaluation of vulnerability of Joints}
We also performed a study of vulnerability of different joints present in the COCO Keypoint benchmark. Table \ref{table:COCO_joints} shows the results of vulnerability of different joints under IGSM-U-10 attacks. We again find the the joints present in the leg are most vulnerable

\section{Results on application of Simple Defense tactics}

Here we present result on application of simple defense strategies such as flipping and gaussian blurring. Table \ref{table:untarDefense} and \ref{table:universalDefense} show the results of flipping and gaussian blurring on Image dependent \& Image Agnostic Perturbations respectively.

\section{Human Skeleton Visualizations}
Figures 7-13 show the results of various adversarial attacks on different images of MPII benchmark. Fig \ref{fig:untargeted_vis} show the predictions of untargeted attacks which Fig \ref{univpdfs_pyranet}, \ref{univpdfs_newell}, \ref{univpdfs_attention}, \ref{univpdfs_shg}, \ref{univpdfs_chained} and \ref{univpdfs_deeppose} show predictions of different models subject to universal perturbations. We find that the predictions corresponding to universal perturbations on a single model look alike. On closer investigation we also found that these predictions are inspired by the humanish figure present in the respective universal noise. 

\section{Evaluation of 3D Human Pose Estimation}
\label{3d_hpe}
As discussed earlier we find that direct regression based approaches are much more vulnerable than corresponding heatmap based approaches. In 3D-HPE, it is a general scheme to regress the depth of a joint directly using a fully connected layer \cite{Zhou_2017_ICCV}. We also compute adversarial perturbations for 3D Human Pose Estimation networks. Specifically we used pretrained model provided by \cite{Zhou_2017_ICCV} on Human 3.6 dataset. We only computed adversarial perturbation for perturbing the z coordinate. We found that indeed the model was very vulnerable. MPJPE is the standard metric used in 3D-HPE which measures the mean per joint prediction error. The original model had performance of \textbf{60} MPJPE, after applying adversarial perturbations the new MPJPE became \textbf{360}. %Due to unavaiability of more 3D-HPE pretrained models we don't study 3D-HPE systems in more detail. But this 

\begin{figure*}[]
\vspace{-1em}
\centering

    \subfloat[2-Stacked Hourglass  \label{fig:uni_2shg}]{
        \includegraphics[width=0.26\linewidth]{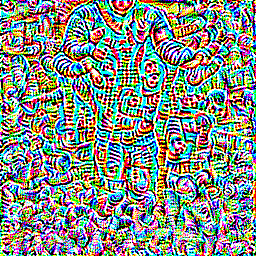}}
    \hfill
    \subfloat[Chained Predictions  \label{fig:uni_chained}]{
        \includegraphics[width=0.26\linewidth]{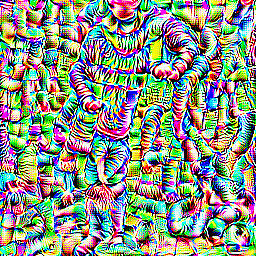}}
    \hfill
    \subfloat[Attention Hourglass  \label{fig:uni_attention}]{
        \includegraphics[width=0.26\linewidth]{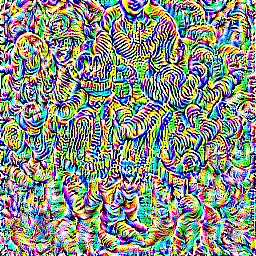}}
    \\
    
 \vspace{-0.025\linewidth}
    
    \subfloat[8-Stacked Hourglass  \label{fig:uni_8shg}]{
        \includegraphics[width=0.26\linewidth]{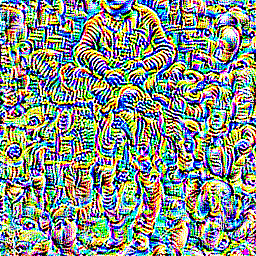}}
    \hfill
    \subfloat[DLCM  \label{fig:uni_DLCM}]{
        \includegraphics[width=0.26\linewidth]{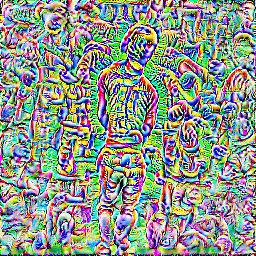}}
    \hfill
    \subfloat[DeepPose  \label{fig:uni_deeppose}]{
        \includegraphics[width=0.26\linewidth]{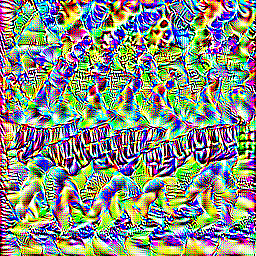}}

\caption{Visualization of image-agnostic universal perturbations, with $\epsilon=16$, for different networks scaled between 0 to 255 for better visualization generated.}

\label{fig:UniversalAdversarial_eps8}
\end{figure*}

\begin{figure*}
\centering

    \subfloat[128 training images  \label{fig:uni_2shg}]{
        \includegraphics[width=0.26\linewidth]{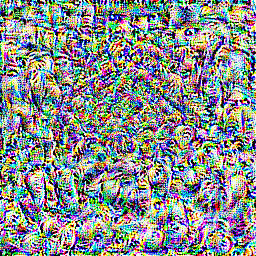}}
    \hfill
    \subfloat[512 training images  \label{fig:uni_chained}]{
        \includegraphics[width=0.26\linewidth]{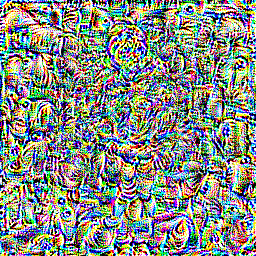}}
    \hfill
    \subfloat[1250 training images  \label{fig:uni_attention}]{
        \includegraphics[width=0.26\linewidth]{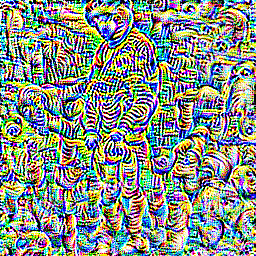}}
    \\
\vspace{-0.025\linewidth}
    \subfloat[2500 training images  \label{fig:uni_8shg}]{
        \includegraphics[width=0.26\linewidth]{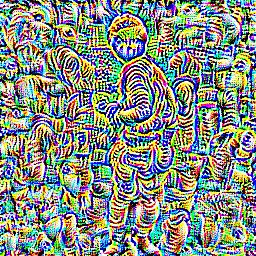}}
    \hfill
    \subfloat[5000 training images  \label{fig:uni_DLCM}]{
        \includegraphics[width=0.26\linewidth]{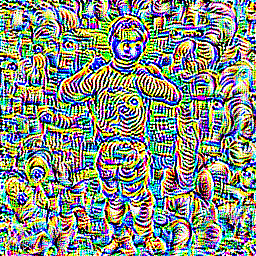}}
        \hfill
    \subfloat[17500 training images  
    \label{fig:uni_deeppose}]{
        \includegraphics[width=0.26\linewidth]{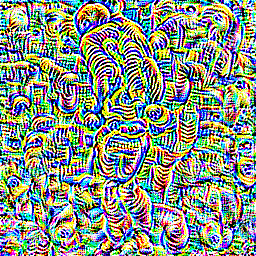}}
\caption{Visualization of the image-agnostic universal perturbations generated from the 8-Stacked-Hourglass model using a limited number of training samples. Note that as amount of data increased the perturbation look semantically more meaningful}
\label{fig:UniversalAdversarial_small}
\end{figure*}

\begin{figure*}
\centering

    \subfloat{
        \includegraphics[height=0.3\linewidth]{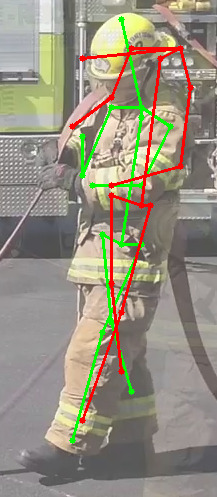}}
    \hfill
    \subfloat{
        \includegraphics[height=0.3\linewidth]{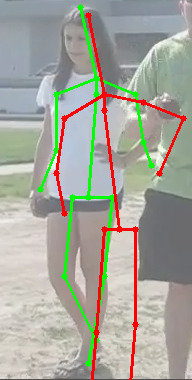}}
    \hfill
    \subfloat{
        \includegraphics[height=0.3\linewidth]{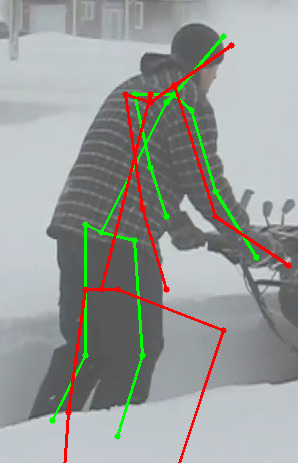}}
    \hfill
    \subfloat{
        \includegraphics[height=0.3\linewidth]{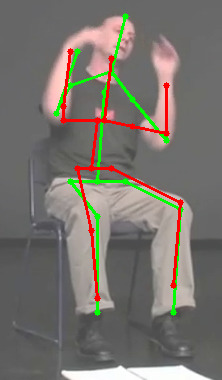}}
    \hfill

\vspace{.5em}

\subfloat{
        \includegraphics[height=0.3\linewidth]{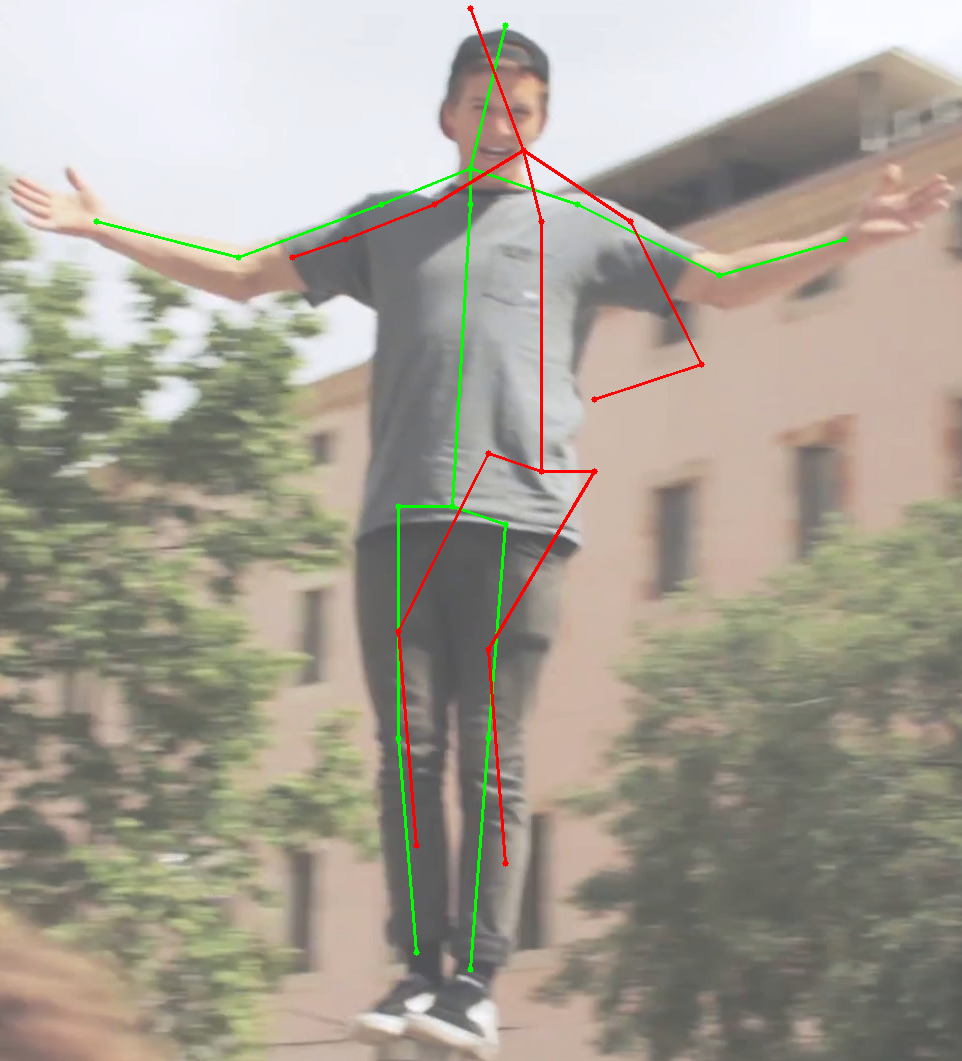}}
    \hfill 
    \subfloat{
        \includegraphics[height=0.3\linewidth]{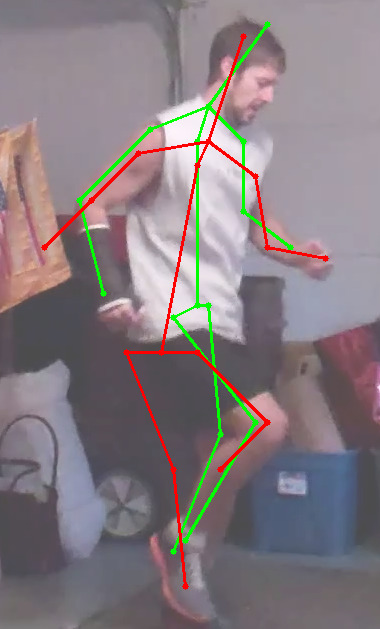}}
    \hfill
    \subfloat{
        \includegraphics[height=0.3\linewidth]{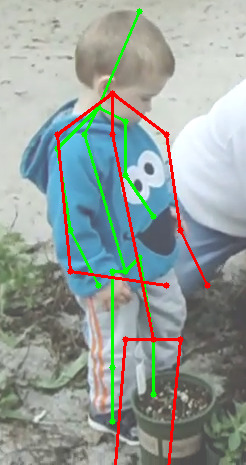}}
    \hfill
    \subfloat{
        \includegraphics[height=0.3\linewidth]{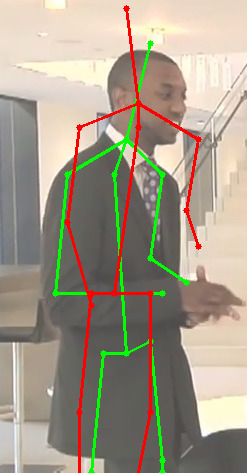}}
    \hfill

\vspace{.5em}

\subfloat{
        \includegraphics[height=0.3\linewidth]{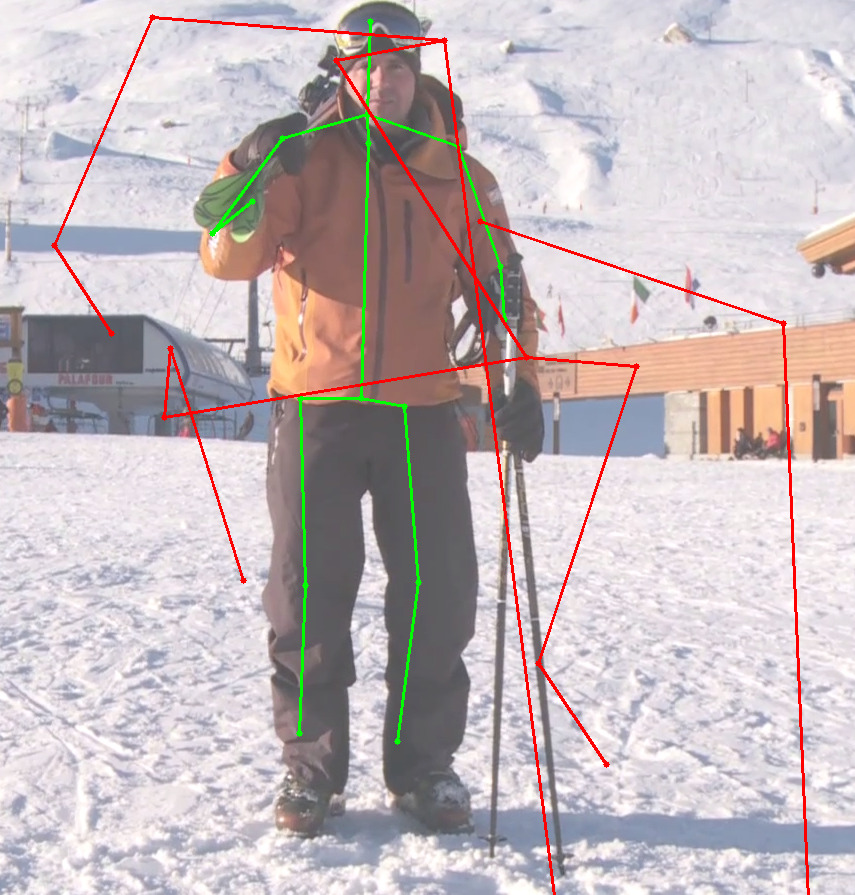}}
    \hfill
    \subfloat{
        \includegraphics[height=0.3\linewidth]{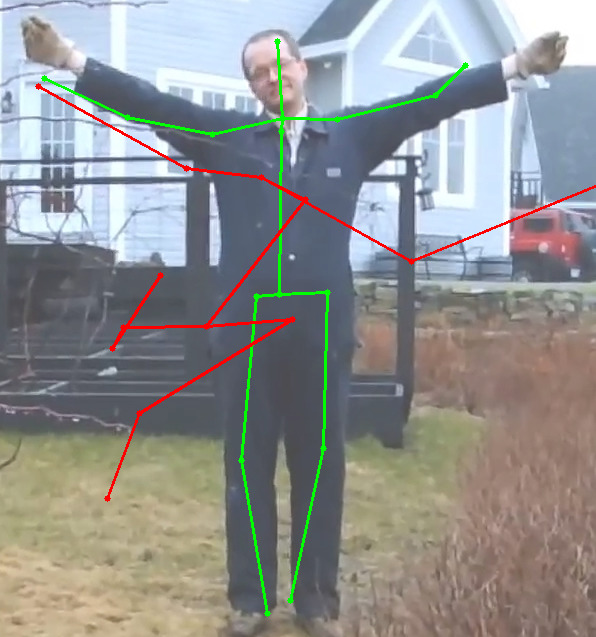}}
    \hfill
    \subfloat{
        \includegraphics[height=0.3\linewidth]{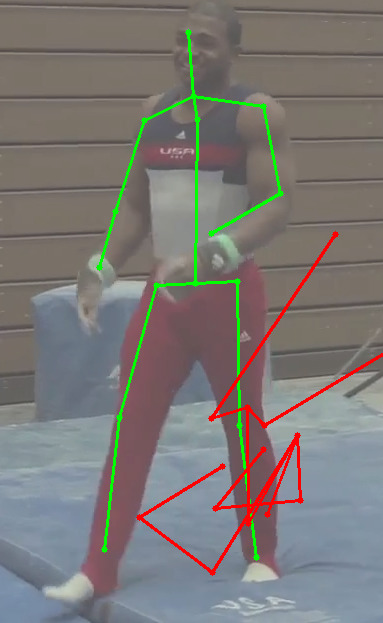}}
    \hfill
    \subfloat{
        \includegraphics[height=0.3\linewidth]{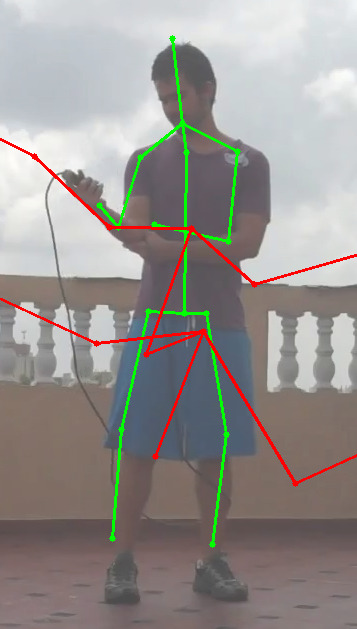}}
    \hfill

\vspace{.5em}

\subfloat{
        \includegraphics[height=0.3\linewidth]{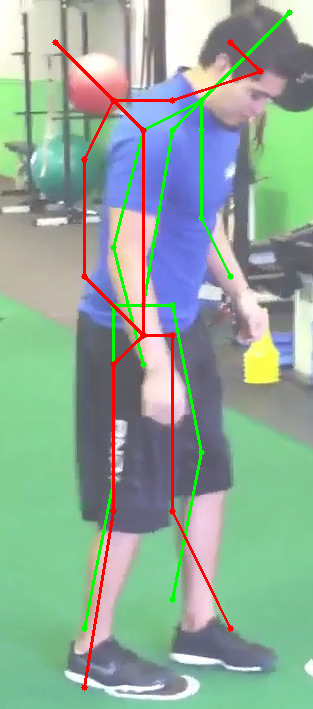}}
    \hfill
    \subfloat{
        \includegraphics[height=0.3\linewidth]{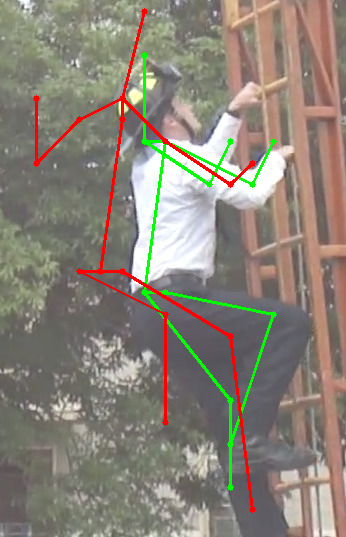}}
    \hfill
    \subfloat{
        \includegraphics[height=0.3\linewidth]{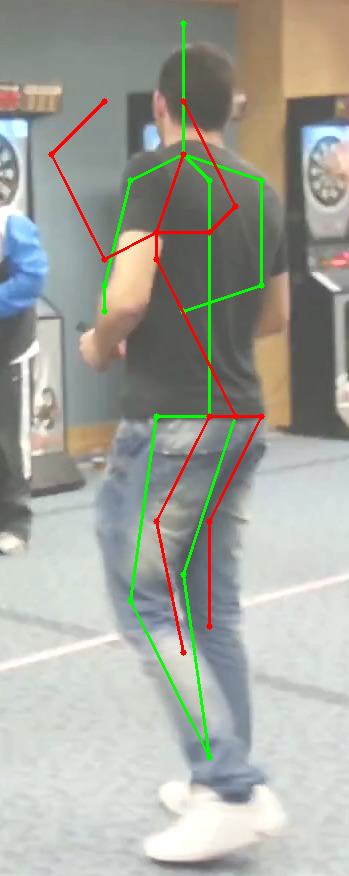}}
    \hfill
    \subfloat{
        \includegraphics[height=0.3\linewidth]{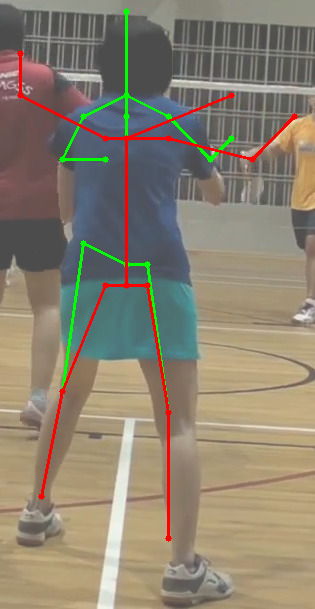}}
    \hfill

\caption{Examples of untargeted adversarial attacks of different model on the MPII benchmark. The images in first row are generated using the Attention model; second row using the 2-Stacked-Hourglass; third row using the DeepPose model; and fourth or the last row using the Chained-Predictions model}
\label{fig:untargeted_vis}
\end{figure*}

\begin{figure*}
\includegraphics[width = \linewidth]{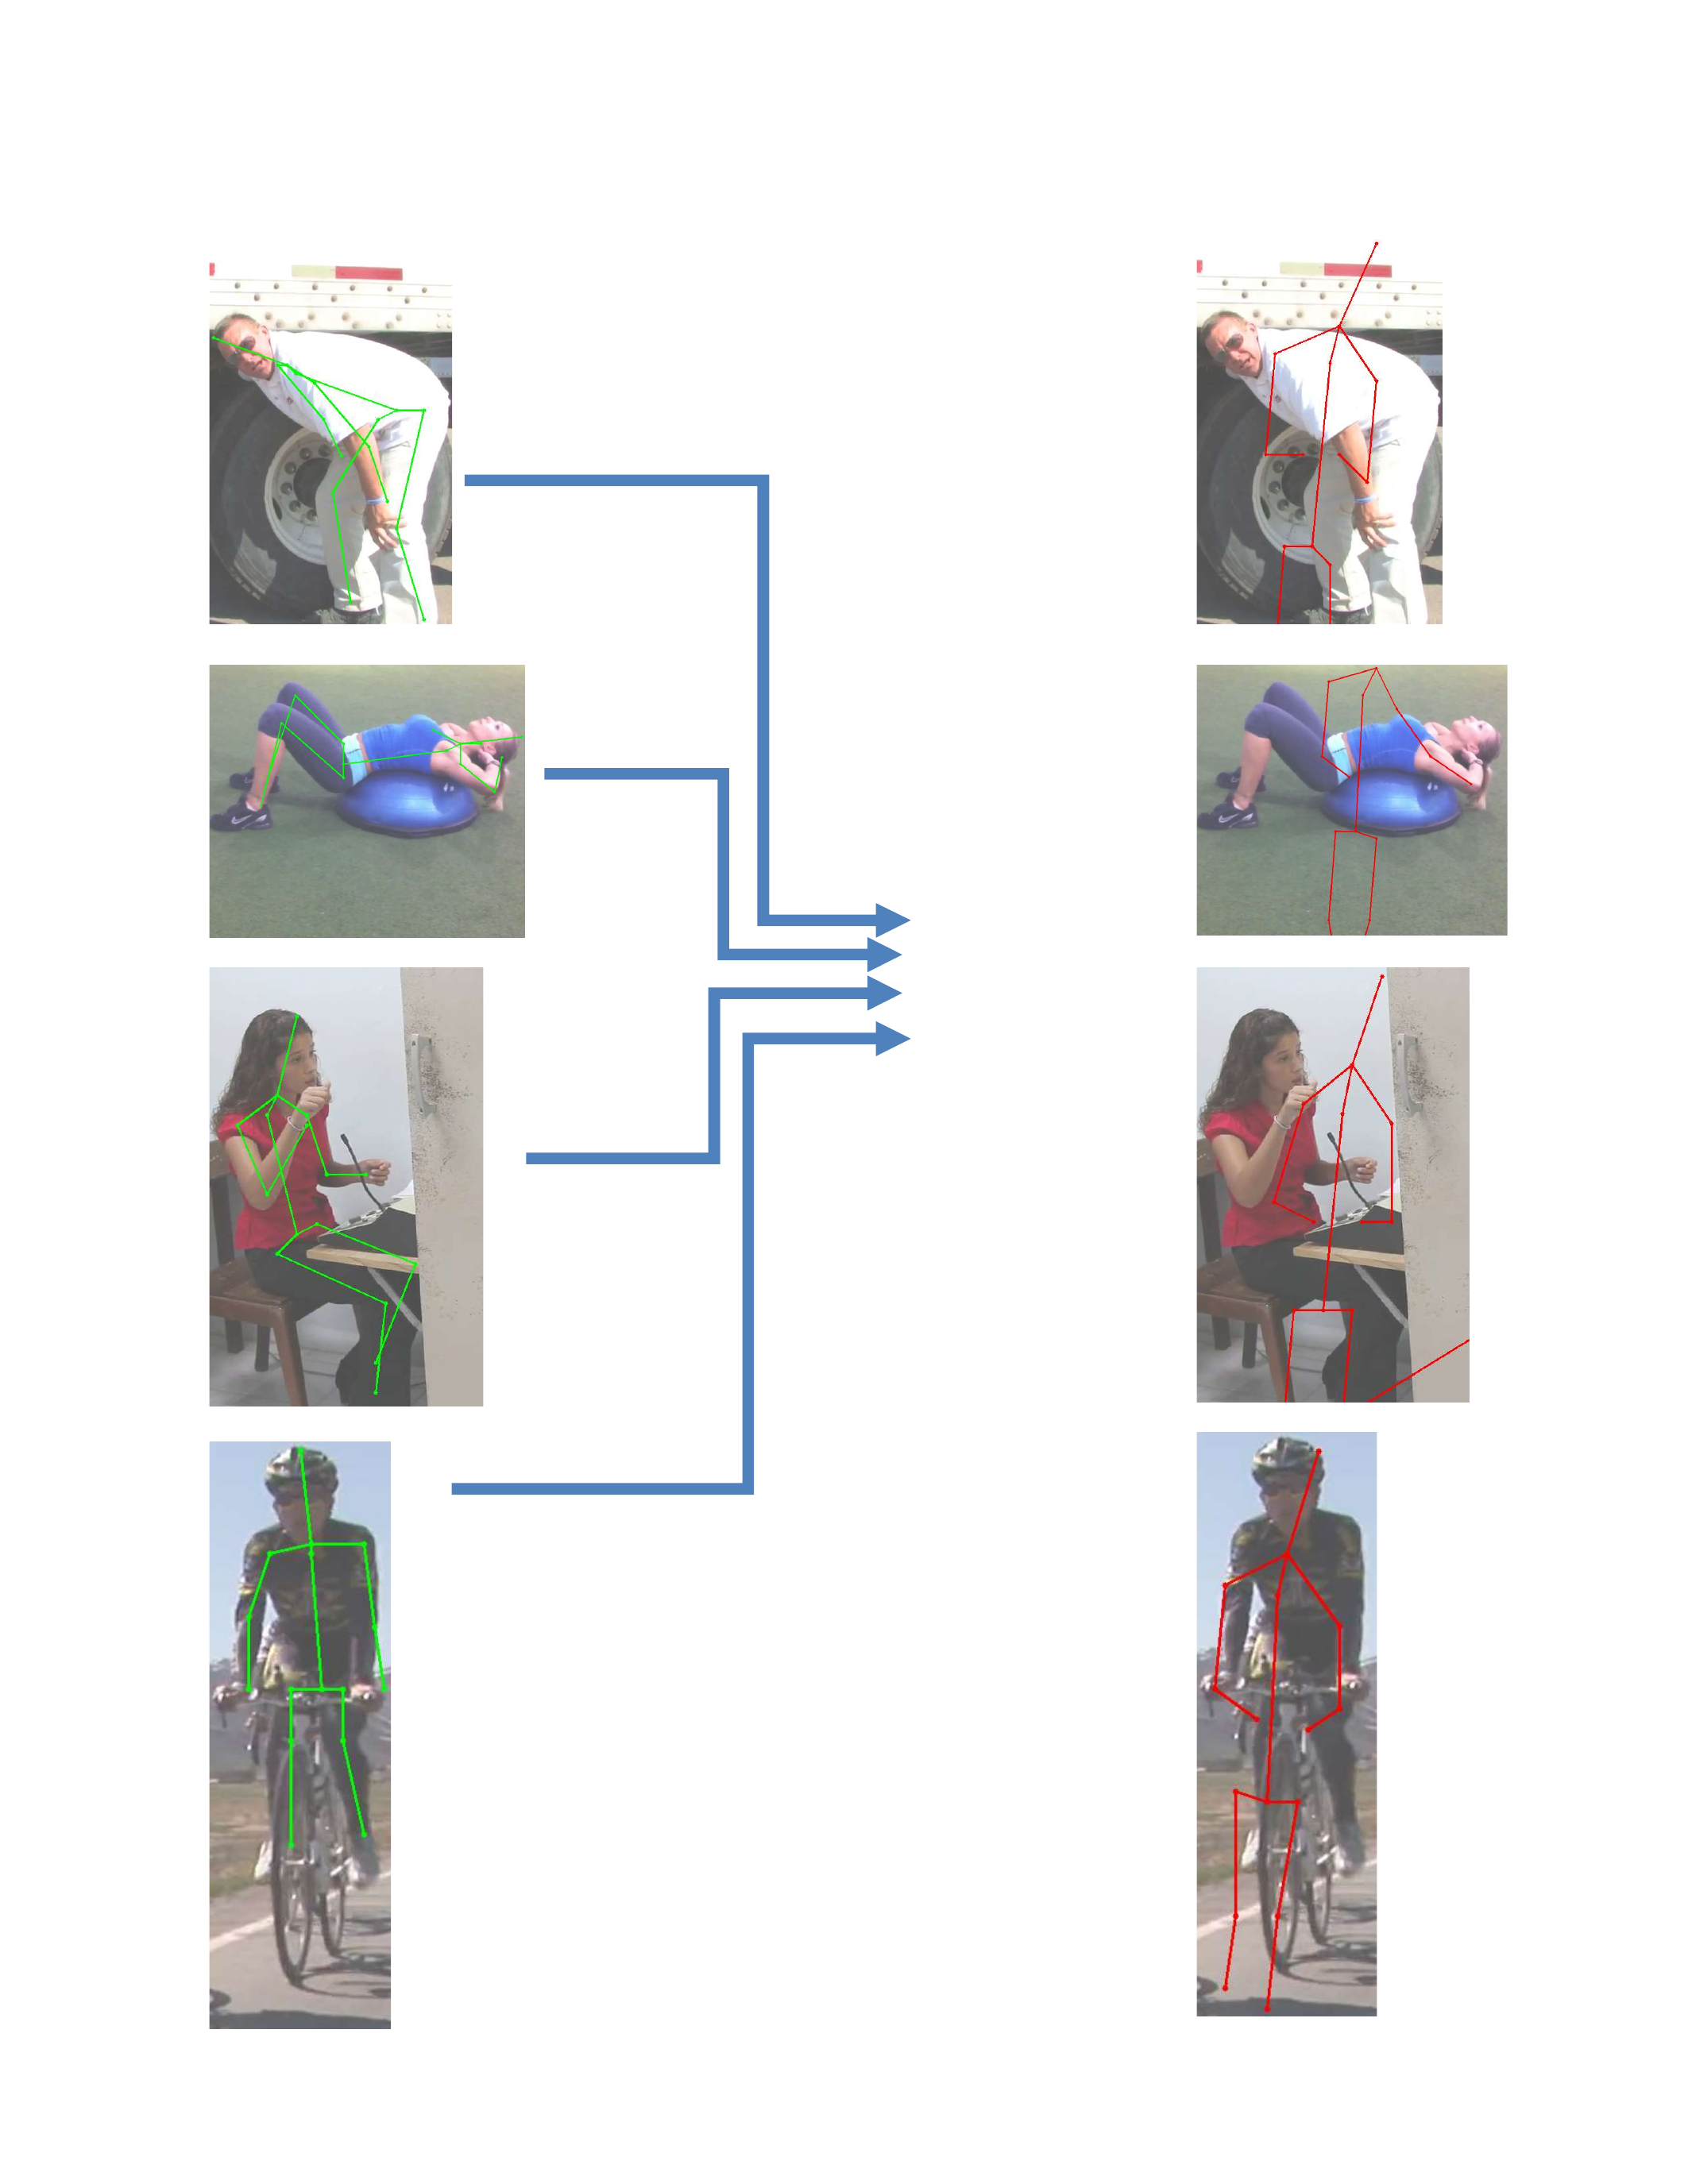}
\caption{Some examples predictions of DLCM model when subject to universal perturbations. All images (left) are subject to same perturbation computed for DLCM and new predictions in (right)}
\label{univpdfs_pyranet}

\end{figure*}

\begin{figure*}
\includegraphics[width = \linewidth]{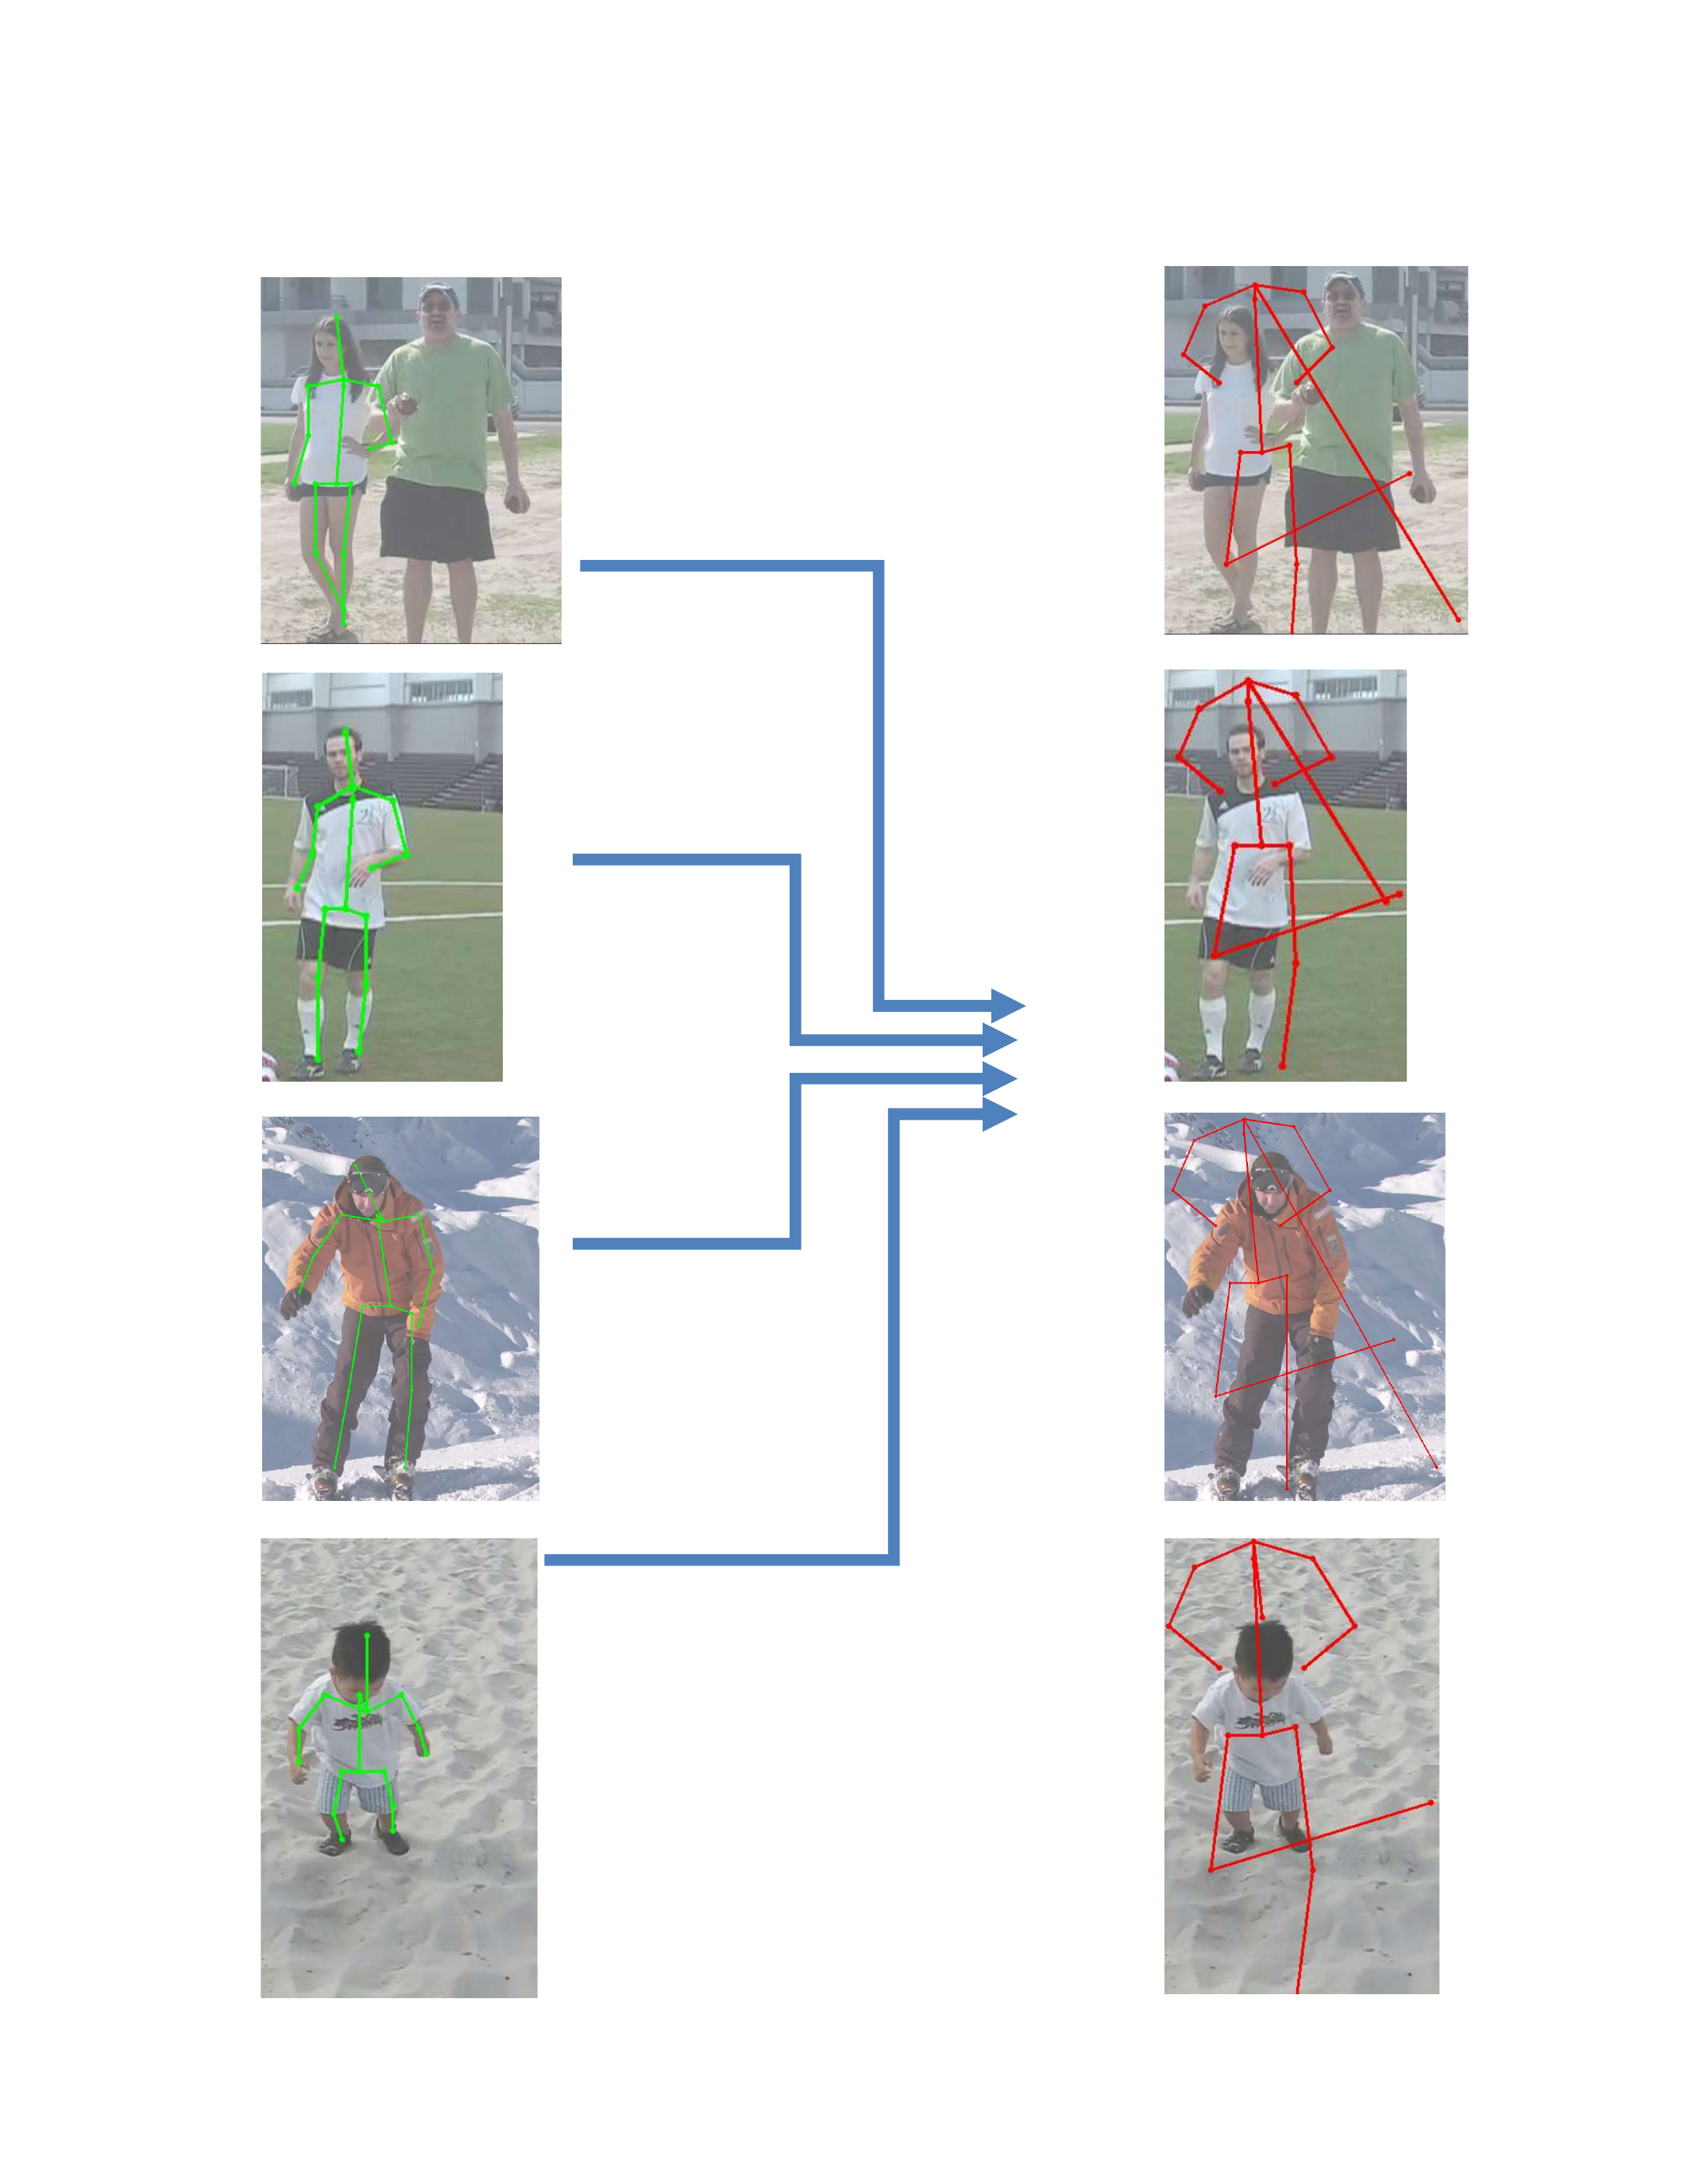}
\caption{Some examples predictions of 8-SHG model when subject to universal perturbations. All images (left) are subject to same perturbation computed for 8-SHG and new predictions in (right)}
\label{univpdfs_newell}

\end{figure*}

\begin{figure*}
\includegraphics[width = \linewidth]{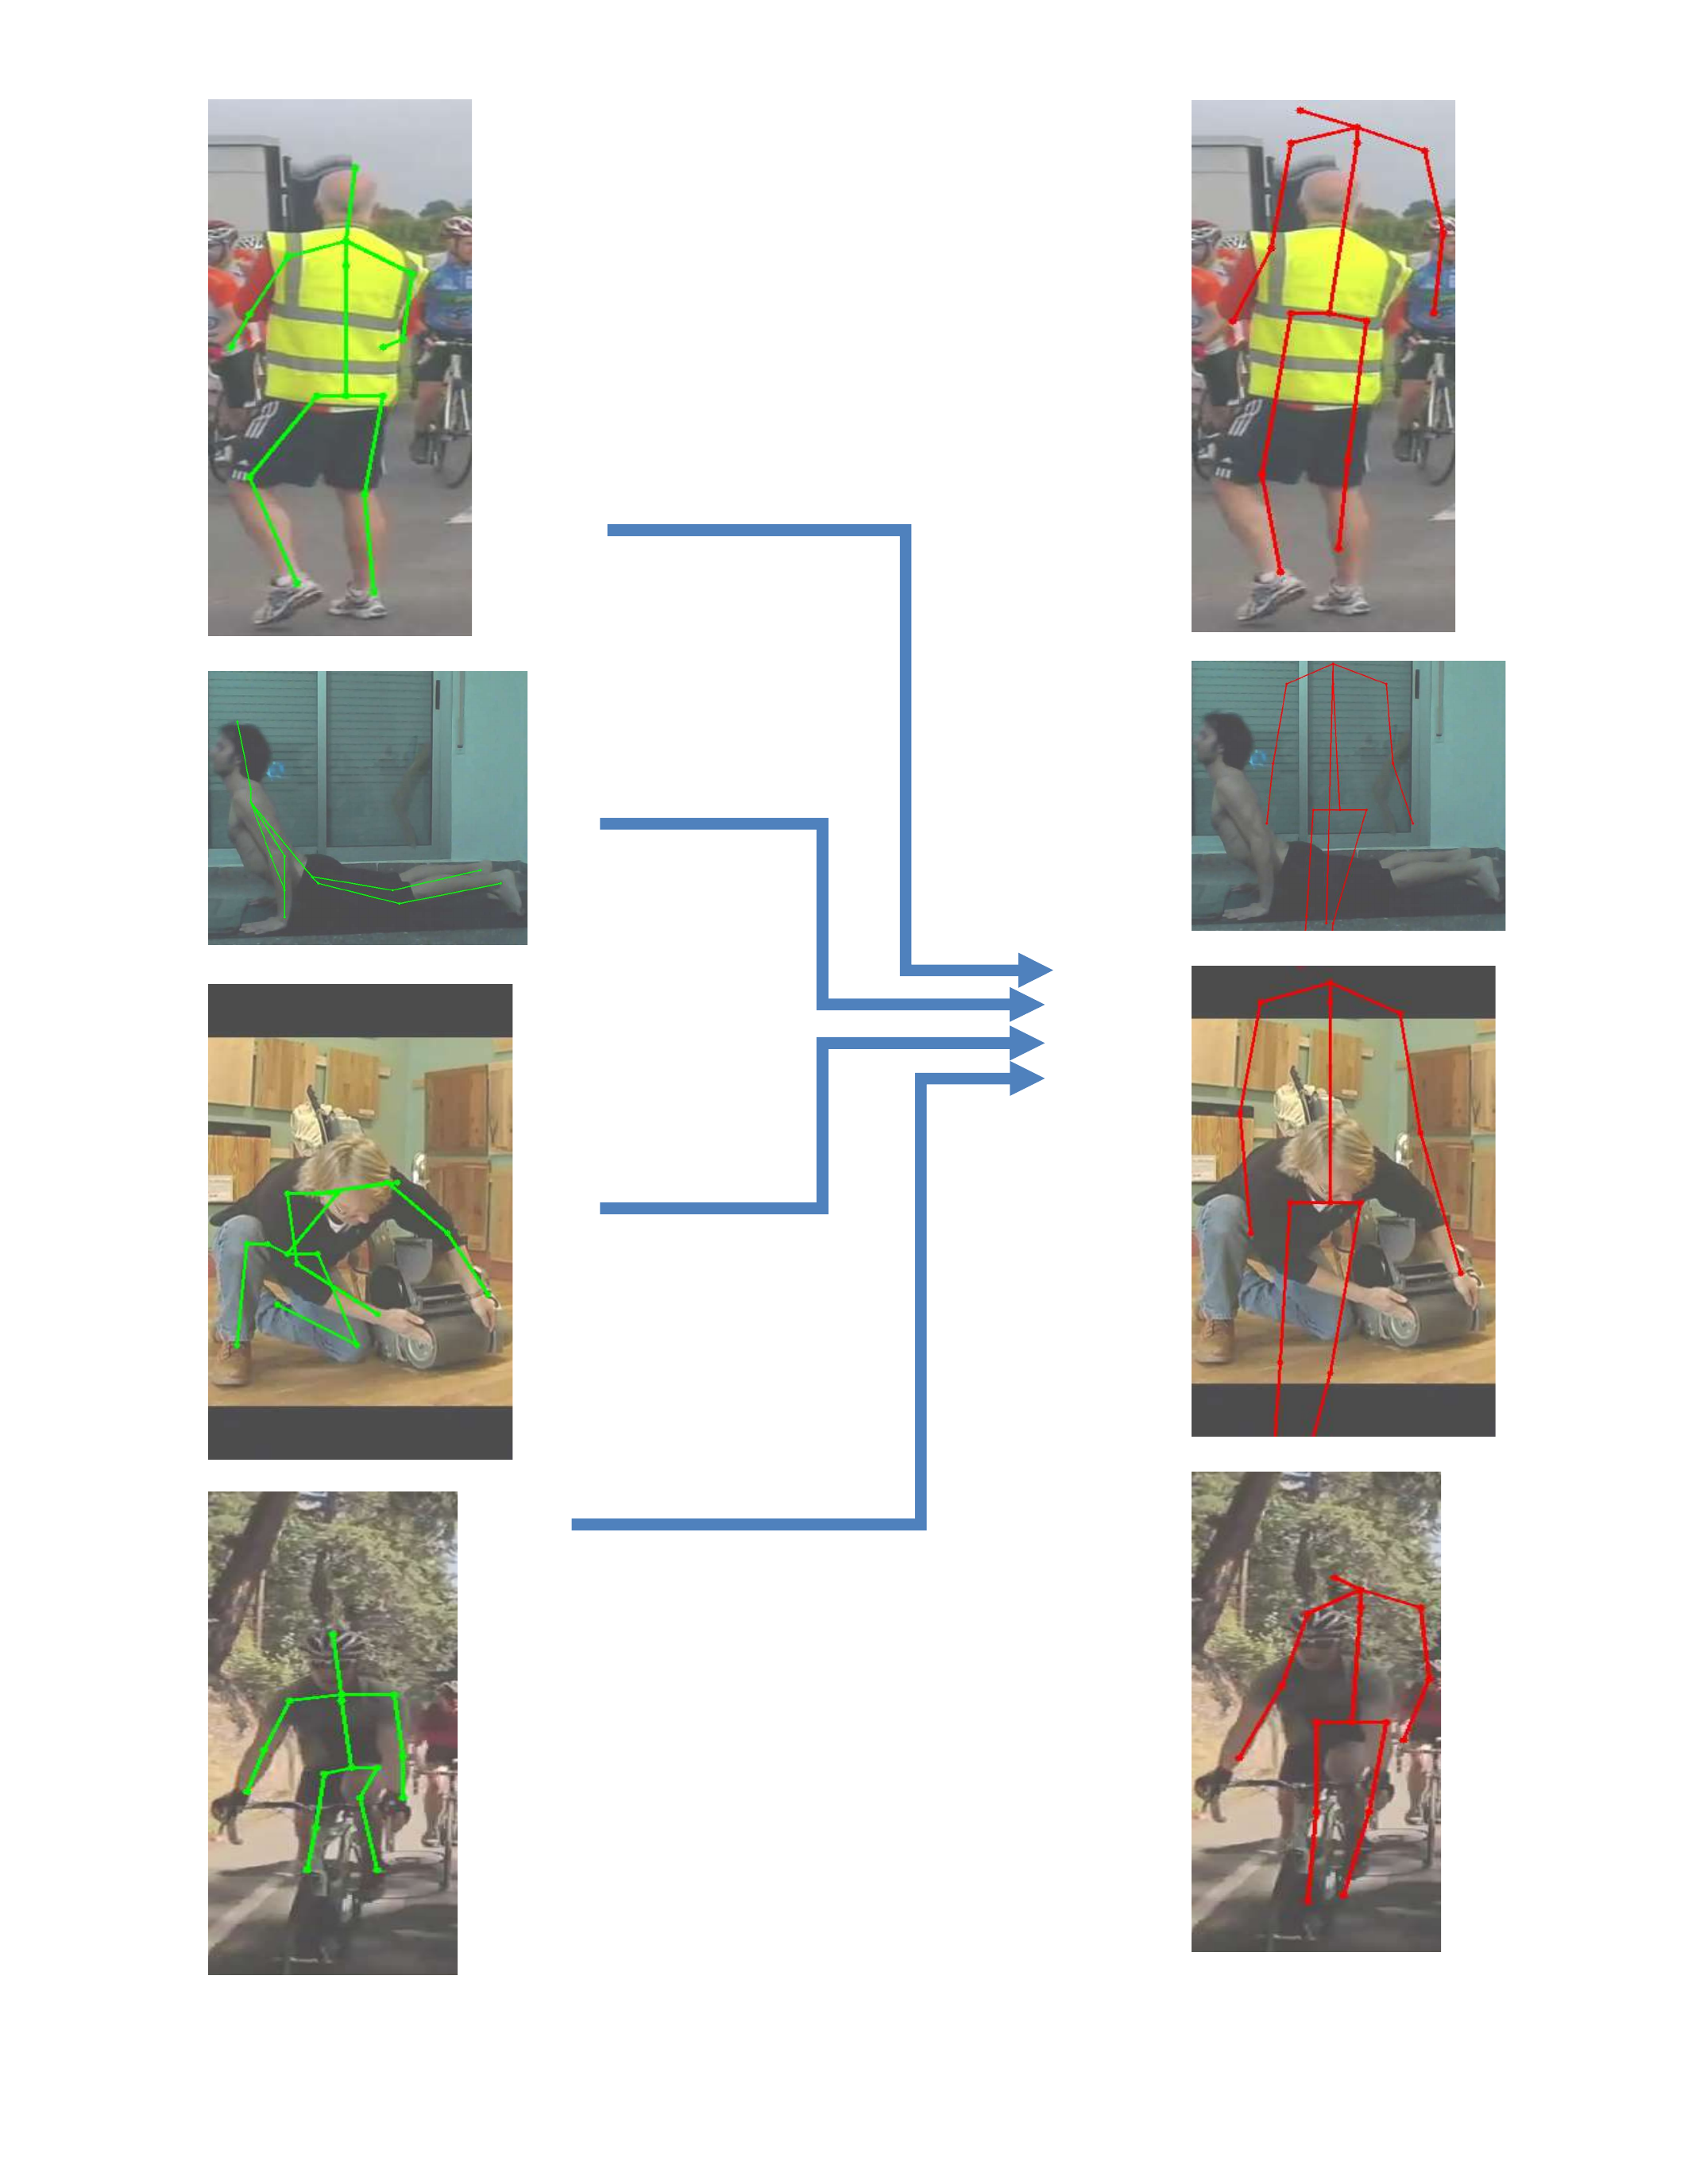}
\caption{Some examples predictions of Attn-HG model when subject to universal perturbations. All images (left) are subject to same perturbation computed for Attn-HG and new predictions in (right)}
\label{univpdfs_attention}

\end{figure*}

\begin{figure*}
\includegraphics[width = \linewidth]{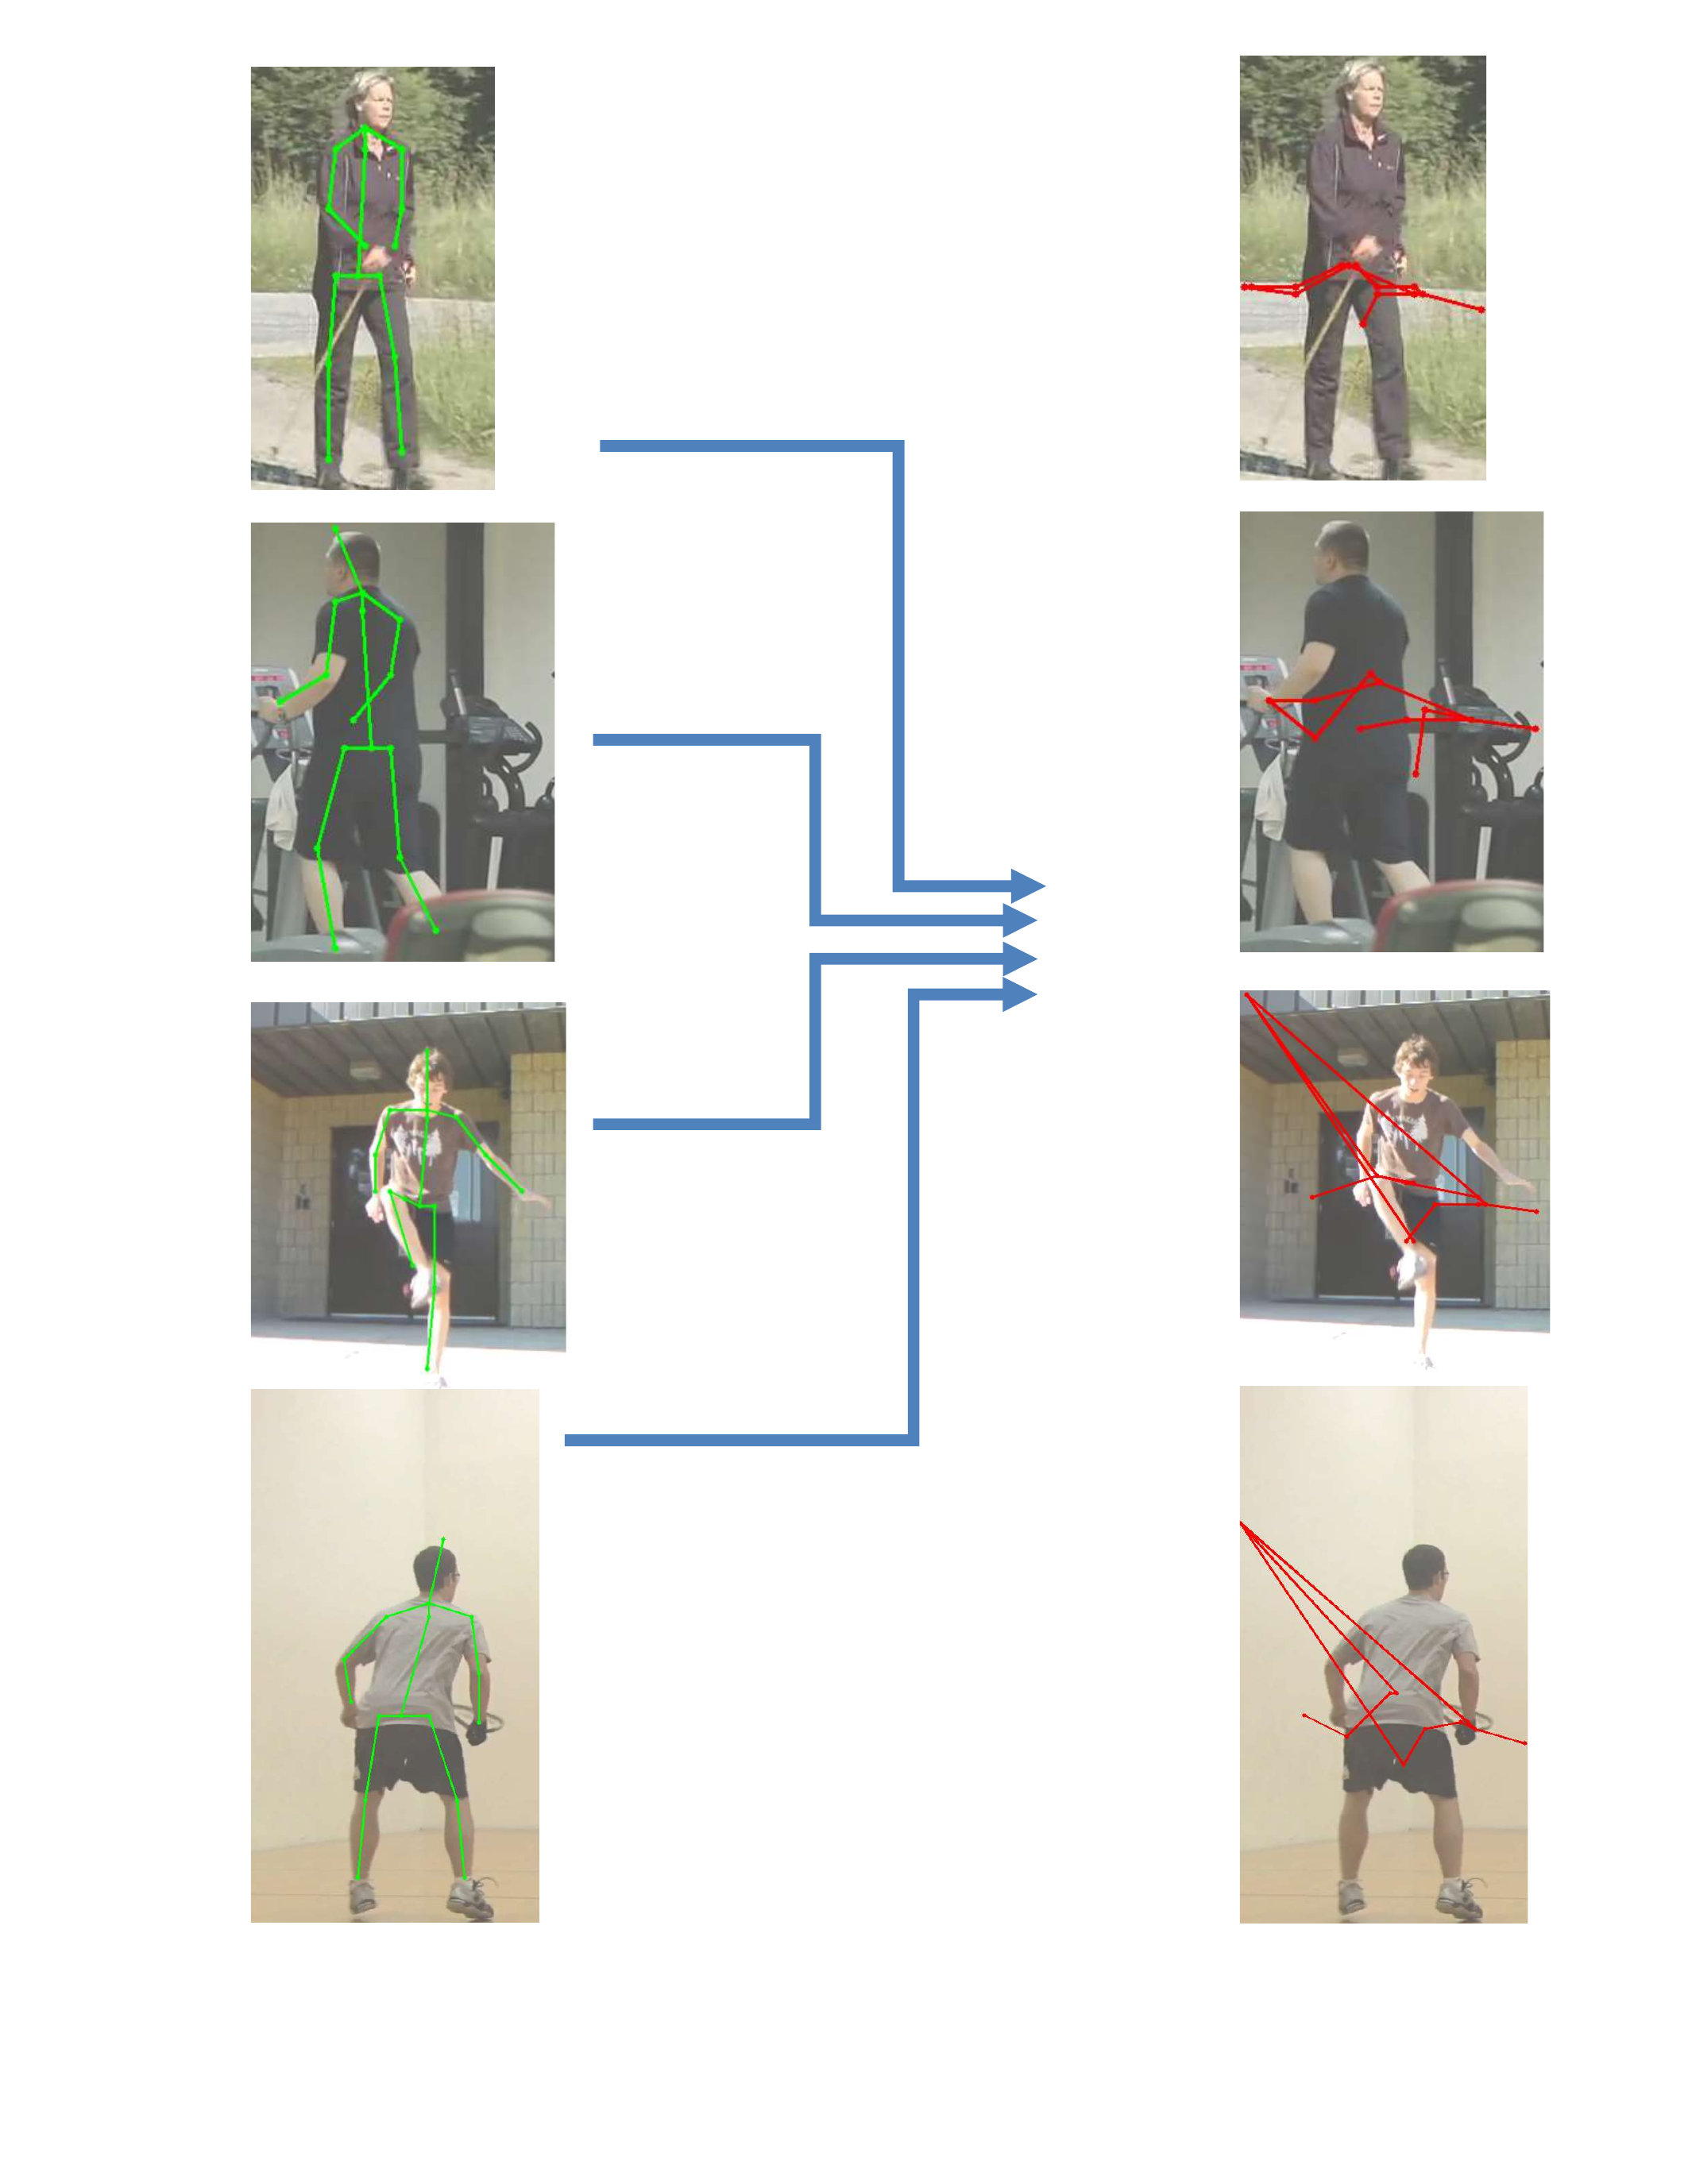}
\caption{Some examples predictions of 2-SHG model when subject to universal perturbations. All images (left) are subject to same perturbation computed for 2-SHG and new predictions in (right)}
\label{univpdfs_shg}

\end{figure*}

\begin{figure*}
\includegraphics[width = \linewidth]{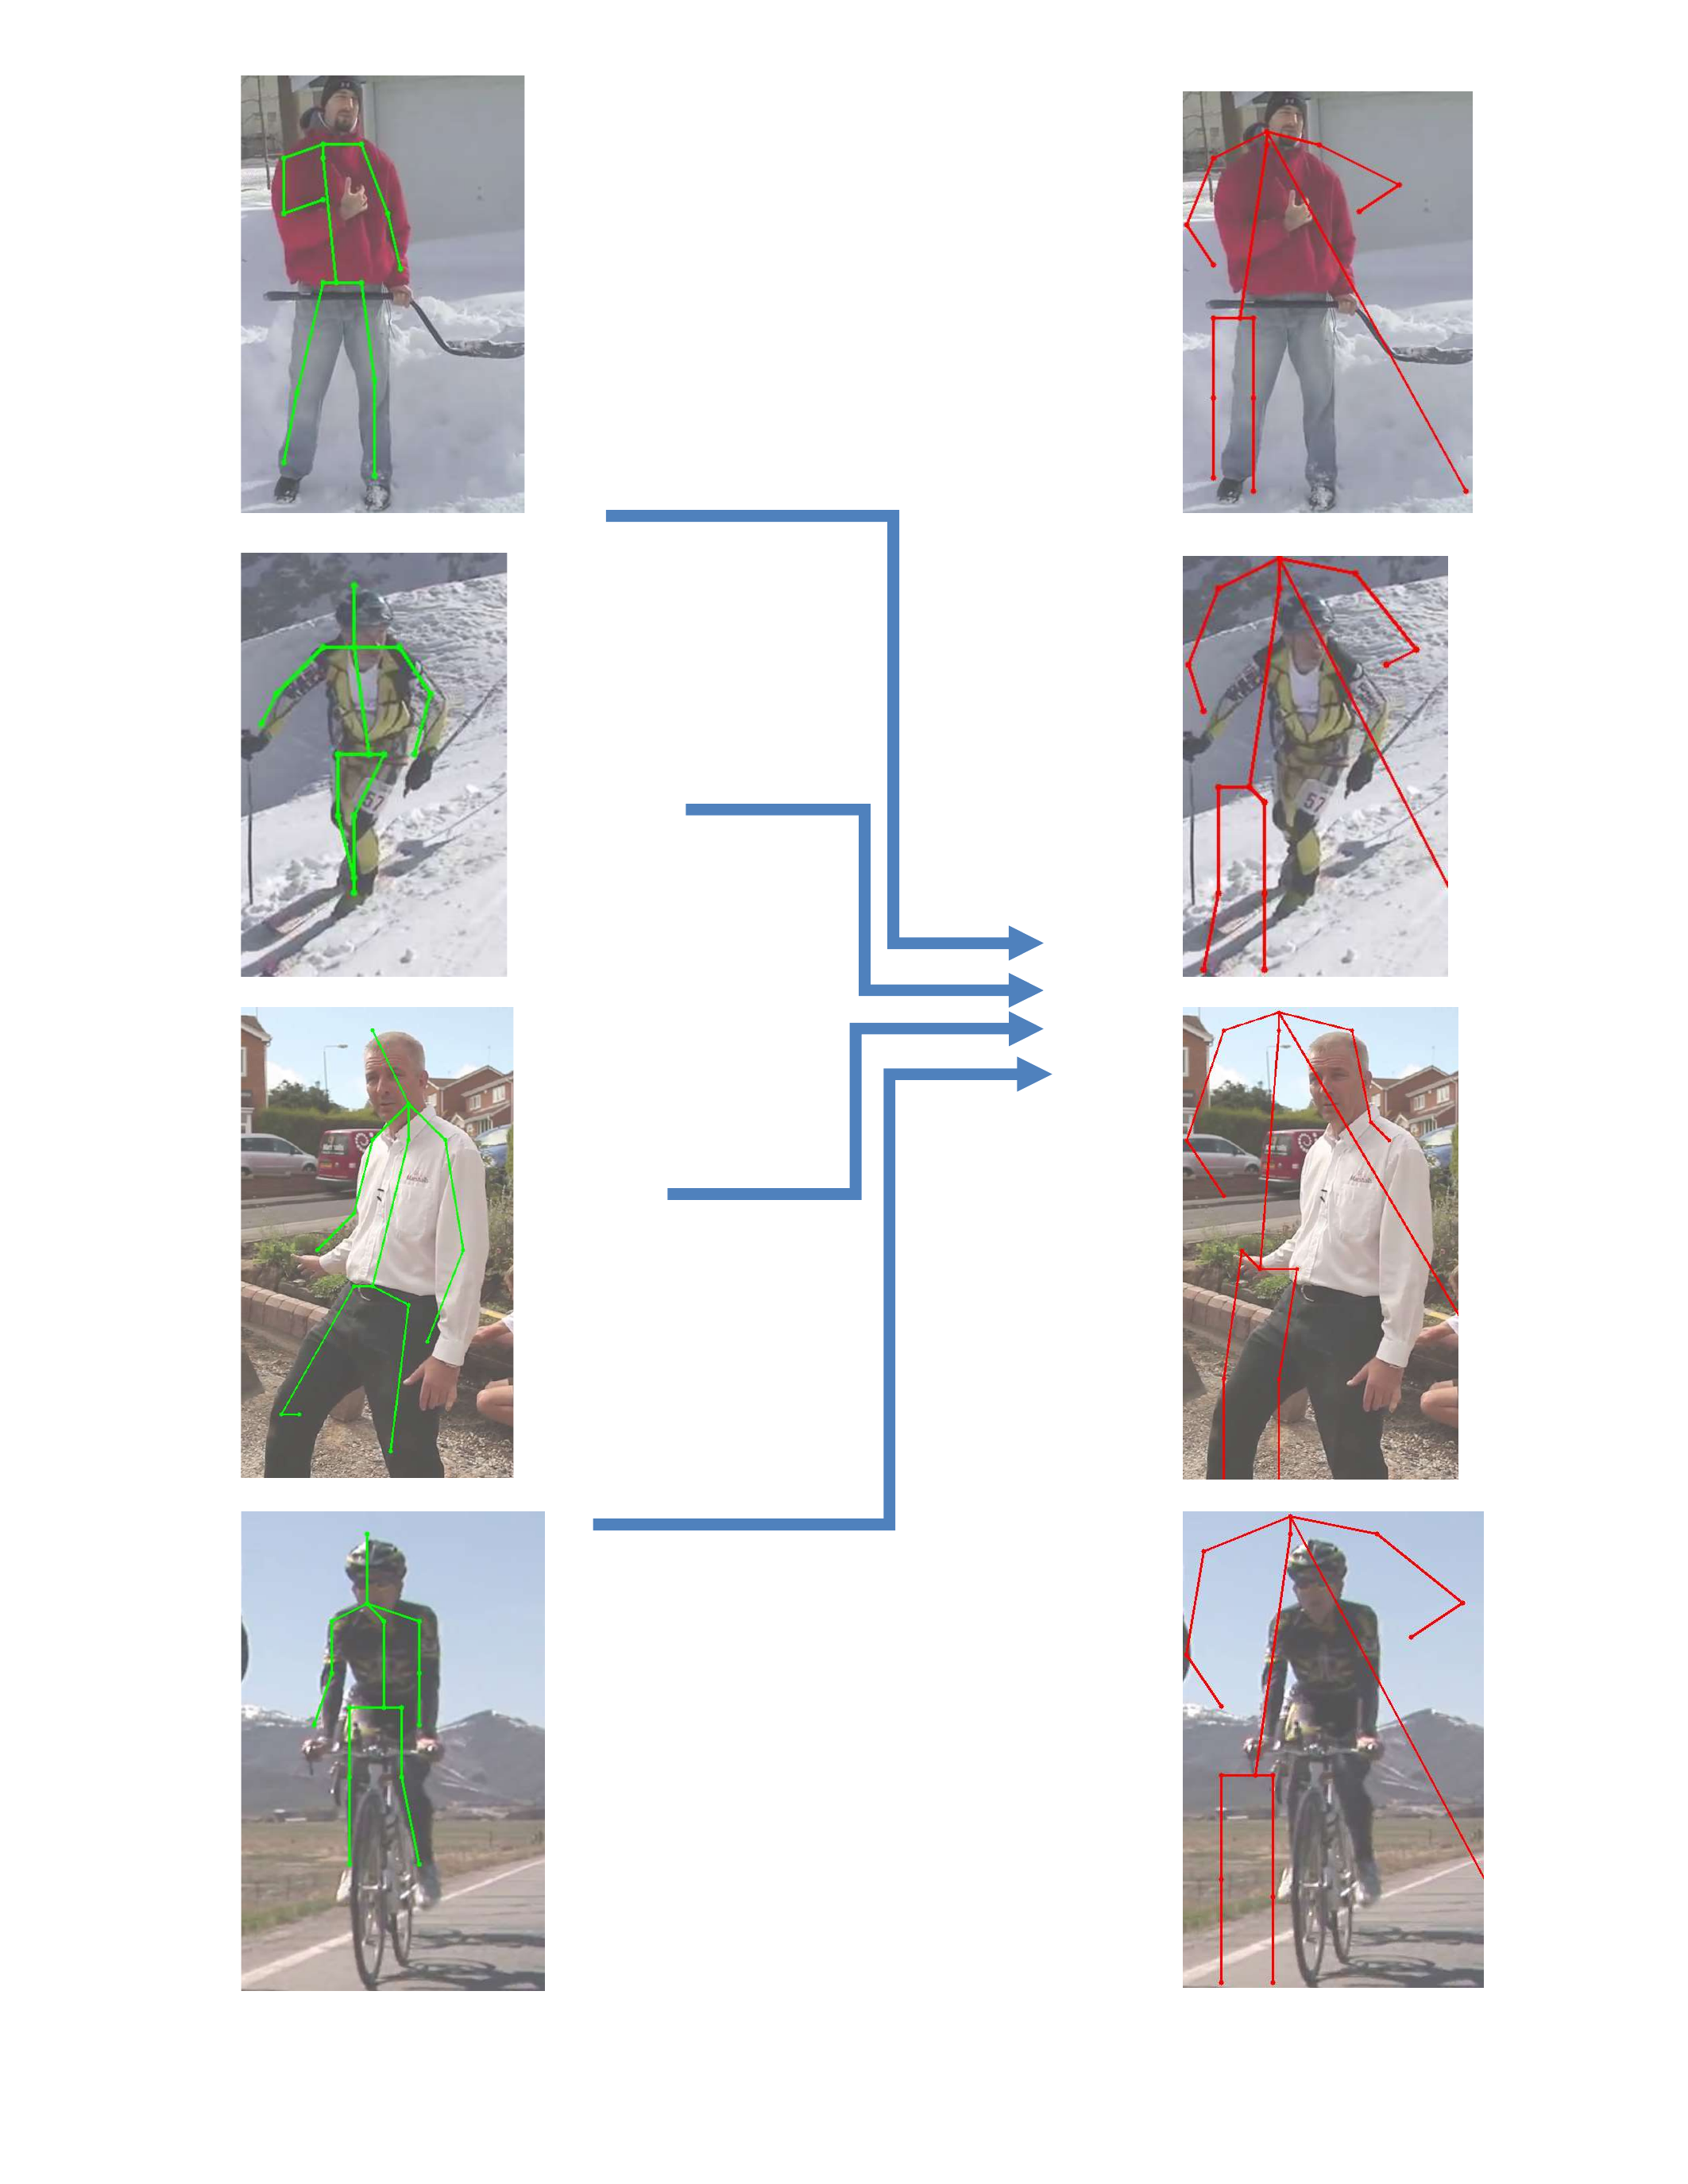}
\caption{Some examples predictions of Chained Predictoions model when subject to universal perturbations. All images (left) are subject to same perturbation computed for Chained Predictions and new predictions in (right)}
\label{univpdfs_chained}
\end{figure*}

\begin{figure*}
\includegraphics[width = \linewidth]{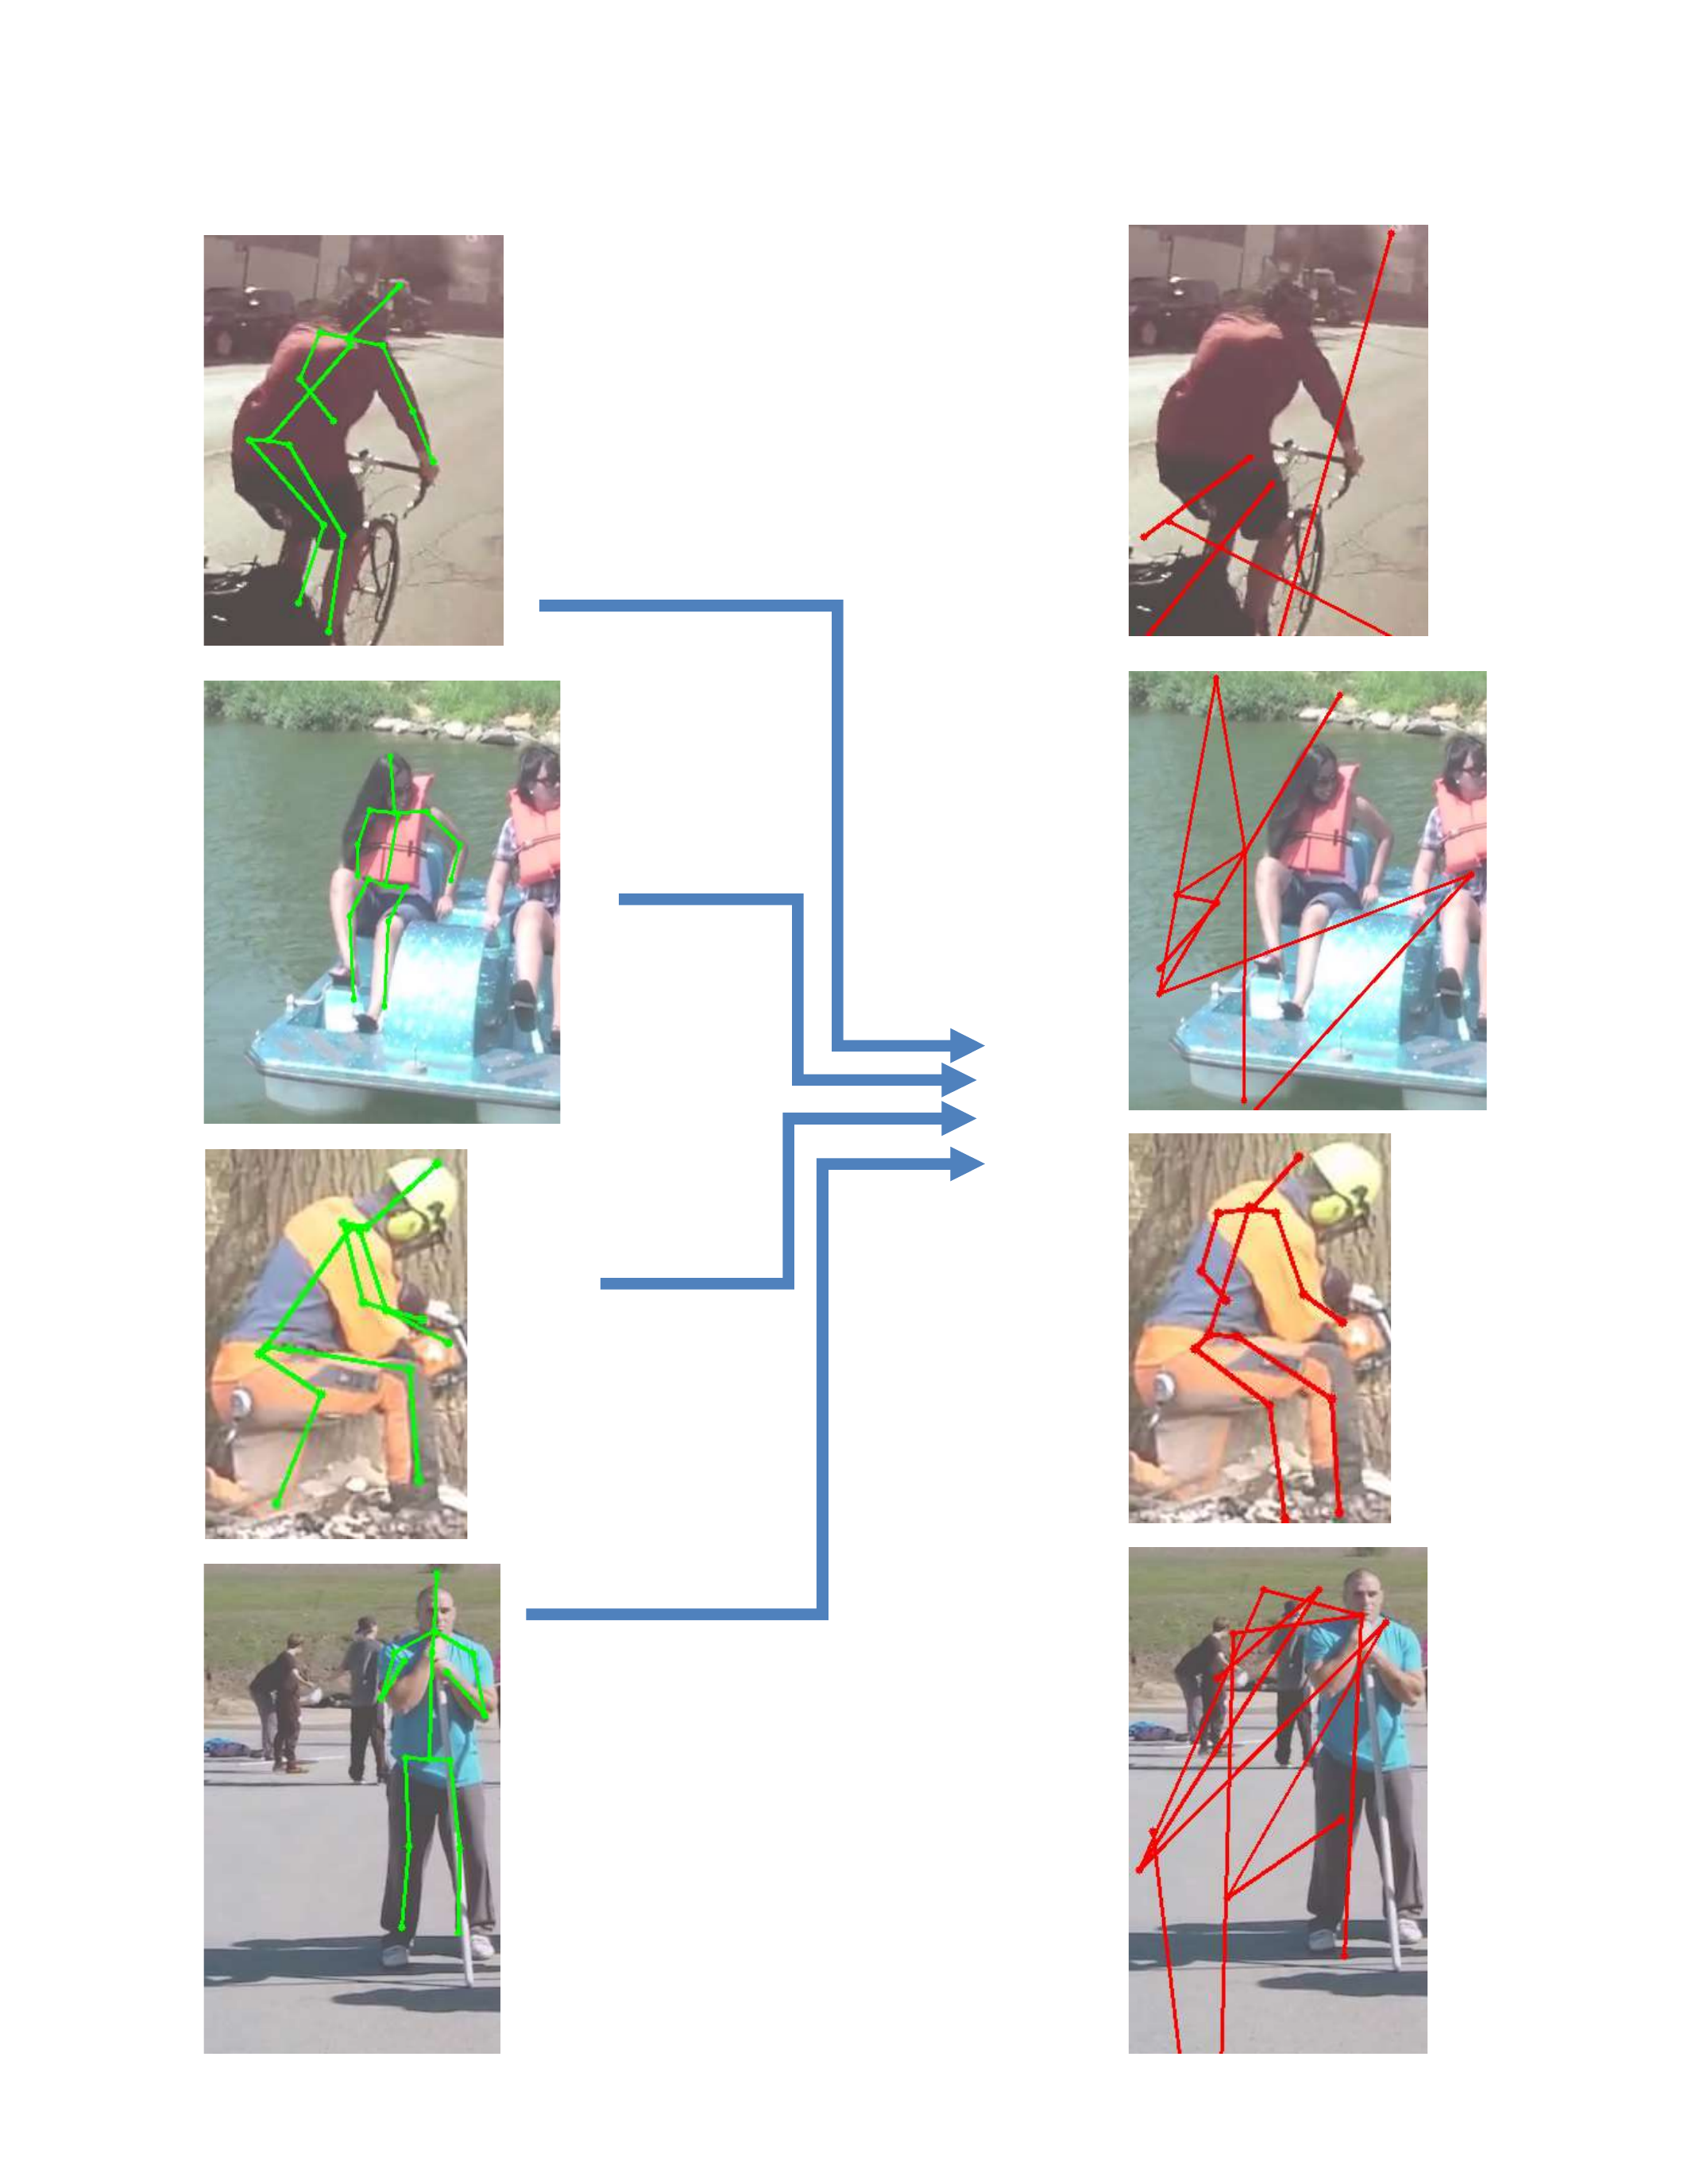}
\caption{Some examples predictions of DeepPose model when subject to universal perturbations. All images (left) are subject to same perturbation computed for DeepPose and new predictions in (right)}
\label{univpdfs_deeppose}
\end{figure*}

%%%%%%%%%%%%%%%%%%%%%%%%%%%%%%%%
\begin{table*}[!h]
\centering
 \begin{tabular}{c c c c c c c c c c} 
 \hline
  & \hspace{-1px}  8-SHG & \hspace{-1px}  atten- & \hspace{-1px}  DLCM & \hspace{-1px}  2HG & \hspace{-1px}  chain- & \hspace{-1px}  Deep- & \hspace{-1px}  8-SHG- & \hspace{-1px}  2-SHG- & \hspace{-1px}  Random  \\ [0.5ex]
& \hspace{-1px}  8-SHG & \hspace{-1px}  tion & \hspace{-1px}  DLCM & \hspace{-1px}  2HG & \hspace{-1px}  cpred & \hspace{-1px}  Pose & \hspace{-1px}  all & \hspace{-1px}  all & \hspace{-1px}  Noise \\ [0.5ex]
 \hline

    8-SHG & \hspace{-1px} 20.4 & \hspace{-1px} 86.57 & \hspace{-1px} 85.28 & \hspace{-1px} 70.15 & \hspace{-1px} 79.9 & \hspace{-1px} 87.42 & \hspace{-1px} 20.4 & \hspace{-1px} 67.3 & \hspace{-1px} 97.27 \\
 
 attention & \hspace{-1px} 79.78 & \hspace{-1px} 16.09 & \hspace{-1px} 85.27 & \hspace{-1px} 75.96 & \hspace{-1px} 79.06 & \hspace{-1px} 87.02 & \hspace{-1px} 73.98 & \hspace{-1px} 68.32 & \hspace{-1px} 96.3 \\
 DLCM & \hspace{-1px} 83.73 & \hspace{-1px} 89.07 & \hspace{-1px} 17.73 & \hspace{-1px} 79.58 & \hspace{-1px} 83.92 & \hspace{-1px} 90.17 & \hspace{-1px} 78.76 & \hspace{-1px} 75.21 & \hspace{-1px} 96.26 \\
 
 2HG & \hspace{-1px} 77.87 & \hspace{-1px} 85.32 & \hspace{-1px} 83.8 & \hspace{-1px} 15.13 & \hspace{-1px} 87.41 & \hspace{-1px} 95.42 & \hspace{-1px} 72.25 & \hspace{-1px} 10.71 & \hspace{-1px} 0.0 \\
 
 chain-pred & \hspace{-1px} 86.19 & \hspace{-1px} 87.73 & \hspace{-1px} 88.24 & \hspace{-1px} 88.33 & \hspace{-1px} 7.6 & \hspace{-1px} 84.59 & \hspace{-1px} 83.47 & \hspace{-1px} 86.76 & \hspace{-1px} 0.0 \\
 
 DeepPose & \hspace{-1px} 78.04 & \hspace{-1px} 78.65 & \hspace{-1px} 80.0 & \hspace{-1px} 86.95 & \hspace{-1px} 57.6 & \hspace{-1px} 5.67 & \hspace{-1px} 76.6 & \hspace{-1px} 85.43 & \hspace{-1px} 0.0 \\
 \hline
 \end{tabular}
 \caption{Table containing performance of models on image-dependent black box attacks on MPII dataset. A row corresponds to the performance of a single model being attacked by different models in different columns}
 \label{BlackBoxTable}
\end{table*}

\begin{table*}[!h]
\begin{center}
\begin{tabular}{l|c}
\hline
Model & PCKh on Validation Set \\
\hline
8-Stacked-Hourglass &88.51\\
Attenion & 87.94\\
DLCM & 89.46\\
2-Stacked-Hourglas & 87.62\\
Chained Predictions & 81.76\\
DeepPose & 56.97\\
\hline
\end{tabular}
\end{center}
\caption{Table showing the original performance of the models on the validation set (for the MPII dataset) under our experimental setup}
\label{table:originalPerformance}
\end{table*}

%%%%%%%%%%%%%%%%%%%%%%%%%%%%%%%%

%----------------------------------------------------------------------------

%----------------------------------------------------------------------------
% \begin{table*}[h]
% \centering
% \begin{tabular}{c c c c c c c c c}
% \hline
% Model & 0.25 & 0.5 & 1 & 2 & 4 & 8 & 16 & 32\\[0.5ex]
% \hline
% DeepPose & 60.27 & 46.01 & 32.69 & 20.17 & 10.48 & 5.99 & 3.96 & 3.06\\
% Chained & 83.9 & 69.66 & 50.25 & 30.38 & 15.48 & 7.6 & 4.93 & 3.49\\
% 2-SHG & 81.48 & 69.52 & 55.11 & 39.75 & 26.16 & 15.13 & 8.07 & 4.29\\
% 2-SHG-ALL & 79.5 & 64.5 & 47.2 & 31.66 & 19.43 & 10.71 & 5.45 & 3.31\\
% ResDec-Pre & 91.07 & 82.17 & 67.49 & 48.85 & 30.82 & 17.33 & 9.27 & 5.25\\
% ResDec-NoPre & 91.1 & 82.73 & 68.05 & 47.81 & 28.45 & 14.19 & 7.23 & 4.39\\
% 8-SHG & 81.34 & 70.54 & 57.36 & 44.08 & 31.42 & 20.39 & 11.91 & 5.5\\
% 8-SHG-ALL & 81.52 & 69.79 & 55.41 & 40.34 & 26.33 & 15.2 & 8.68 & 4.21\\
% Attn-HG & 79.23 & 66.67 & 51.48 & 36.55 & 25.36 & 16.09 & 10.42 & 5.19\\
% DLCM & 80.53 & 69.36 & 56.02 & 42.19 & 29.3 & 17.72 & 10.86 & 5.12\\
% \hline
% \end{tabular}
% \vspace{0.3em}
% \caption{\textbf{Relative PCKh} results for different $\epsilon$ values for \textbf{IGSM-U-100} attacks on all models}
% \label{table:UI_10}
% \end{table*}

%----------------------------------------------------------------------------
\begin{table*}[t]
\centering
\begin{tabular}{c c c c c c c c c}
\hline
Model & 0.25 & 0.5 & 1 & 2 & 4 & 8 & 16 & 32\\[0.5ex]
\hline
DeepPose & 86.9 & 72.01 & 48.07 & 20.99 & 8.99 & 6.83 & 7.14 & 7.01\\
Chained & 94.73 & 86.04 & 70.02 & 45.15 & 21.7 & 9.69 & 5.88 & 4.81\\
2-SHG & 91.02 & 79.45 & 60.86 & 39.61 & 24.12 & 15.39 & 10.6 & 6.59\\
2-SHG-ALL & 89.68 & 68.56 & 35.68 & 15.63 & 8.77 & 5.67 & 4.28 & 3.6\\
ResDec-Pre & 97.23 & 93.38 & 84.55 & 66.22 & 39.68 & 19.67 & 11.14 & 7.65\\
ResDec-NoPre & 97.13 & 93.67 & 84.67 & 65.24 & 36.99 & 17.32 & 9.98 & 7.05\\
8-SHG & 93.76 & 86.58 & 72.27 & 50.62 & 31.72 & 18.5 & 11.92 & 8.12\\
8-SHG-ALL & 89.58 & 74.5 & 49.27 & 26.6 & 14.18 & 9.11 & 6.4 & 4.98\\
Attn-HG & 91.05 & 80.21 & 62.38 & 44.97 & 32.29 & 22.33 & 16.94 & 11.91\\
DLCM & 91.39 & 84.1 & 71.56 & 29.66 & 33.93 & 21.64 & 14.74 & 10.57\\
    
\hline
\end{tabular}

\vspace{0.3em}
\caption{\textbf{Relative PCKh} results for different $\epsilon$ values for \textbf{IGSM-U-20} attacks on all model}
\label{table:UI_20}
\end{table*}

%----------------------------------------------------------------------------
\begin{table*}[!h]
\centering
\begin{tabular}{c c c c c c c c c}
\hline
Model & 0.25 & 0.5 & 1 & 2 & 4 & 8 & 16 & 32\\[0.5ex]
\hline
DeepPose & 7.68 & 13.11 & 26.18 & 52.91 & 75.51 & 79.73 & 76.69 & 72.95\\
Chained & 5.62 & 9.45 & 17.9 & 34.05 & 56.17 & 72.61 & 80.36 & 82.81\\
2-SHG & 5.21 & 10.13 & 21.69 & 39.61 & 56.04 & 66.33 & 71.21 & 74.52\\
2-SHG-ALL & 5.35 & 12.85 & 34.36 & 59.86 & 73.87 & 80.47 & 83.76 & 85.0\\
ResDec-Pre & 3.72 & 5.26 & 9.15 & 17.87 & 34.27 & 51.65 & 62.17 & 66.73\\
ResDec-NoPre & 3.56 & 5.02 & 9.16 & 18.99 & 37.75 & 56.61 & 66.28 & 71.05\\
8-SHG & 4.9 & 8.32 & 16.36 & 32.07 & 48.84 & 60.45 & 65.57 & 67.34\\
8-SHG-ALL & 5.8 & 12.01 & 27.41 & 48.62 & 64.12 & 72.65 & 75.69 & 77.6\\
Attn-HG & 5.93 & 10.83 & 21.02 & 34.64 & 47.51 & 55.51 & 59.24 & 61.69\\
DLCM & 6.15 & 10.19 & 17.43 & 63.09 & 43.7 & 52.85 & 56.05 & 54.3\\
\hline
\end{tabular}
\vspace{0.3em}
\caption{\textbf{Absolute PCKh} with respect to the target results for different $\epsilon$ values for \textbf{IGSM-T-20} attacks on all models}
\label{table:TI_20}
\end{table*}

%----------------------------------------------------------------------------

%----------------------------------------------------------------------------
\begin{table*}[!h]
\centering
\begin{tabular}{c c c c c c c c c}
\hline
Model & 0.25 & 0.5 & 1 & 2 & 4 & 8 & 16 & 32\\[0.5ex]
\hline
DeepPose & 68.67 & 59.63 & 51.76 & 45.85 & 42.92 & 42.2 & 41.92 & 37.41\\
Chained & 88.61 & 82.13 & 74.71 & 67.36 & 61.59 & 57.72 & 54.6 & 47.76\\
2-SHG & 89.02 & 84.18 & 79.42 & 75.14 & 72.24 & 69.46 & 64.93 & 48.31\\
2-SHG-ALL & 88.89 & 83.37 & 77.59 & 72.57 & 68.76 & 65.49 & 60.61 & 45.46\\
8-SHG & 89.72 & 85.65 & 82.01 & 79.24 & 77.46 & 75.45 & 68.85 & 40.68\\
8-SHG-ALL & 90.23 & 85.9 & 81.92 & 78.94 & 76.58 & 74.36 & 67.49 & 40.45\\
Attn-HG & 88.52 & 84.7 & 81.33 & 79.58 & 78.52 & 76.77 & 67.83 & 28.2\\
DLCM & 89.68 & 85.84 & 82.15 & 78.99 & 77.4 & 76.1 & 71.66 & 51.87\\
\hline
\end{tabular}
\vspace{0.3em}
\caption{\textbf{Relative PCKh} results for different $\epsilon$ values for \textbf{FGSM-U} attacks on all models}
\label{table:UF}
\end{table*}

%----------------------------------------------------------------------------
\begin{table*}[!h]
\centering
\begin{tabular}{c c c c c c c c c}
\hline
Model & 0.25 & 0.5 & 1 & 2 & 4 & 8 & 16 & 32\\[0.5ex]
\hline
DeepPose & 5.72 & 6.63 & 7.62 & 8.39 & 8.81 & 8.84 & 8.09 & 7.83\\
Chained & 4.53 & 5.48 & 6.6 & 7.65 & 8.32 & 8.7 & 8.76 & 8.44\\
2-SHG & 3.29 & 3.91 & 4.56 & 4.99 & 5.36 & 5.68 & 5.77 & 5.57\\
2-SHG-ALL & 3.29 & 3.93 & 4.73 & 5.29 & 5.91 & 6.06 & 6.1 & 5.92\\
8-SHG & 3.17 & 3.59 & 4.09 & 4.21 & 4.6 & 4.66 & 4.75 & 5.67\\
8-SHG-ALL & 3.21 & 3.82 & 4.27 & 4.82 & 5.1 & 5.27 & 5.42 & 5.69\\
Attn-HG & 3.38 & 3.79 & 4.22 & 4.29 & 4.27 & 4.13 & 4.18 & 3.63\\
DLCM & 3.47 & 4.07 & 4.47 & 4.75 & 5.09 & 4.96 & 5.09 & 5.51\\
\hline
\end{tabular}
\vspace{0.3em}
\caption{\textbf{Absolute PCKh} with respect to the target results for different $\epsilon$ values for \textbf{FGSM-T} attacks on all models}
\label{table:TF}
\end{table*}

%----------------------------------------------------------------------------
\begin{table*}
\centering
\begin{tabular}{c c c c c c c c c}
\hline
Model & 0.25 & 0.5 & 1 & 2 & 4 & 8 & 16 & 32\\[0.5ex]
\hline
DeepPose & 58.09 & 42.11 & 24.8 & 6.7 & 1.1 & 0.23 & 0.1 & 0.1\\
Chained & 83.26 & 66.98 & 42.28 & 16.72 & 3.18 & 0.52 & 0.23 & 0.22\\
2-SHG & 78.54 & 62.69 & 50.59 & 32.4 & 17.31 & 7.13 & 2.27 & 0.53\\
8-SHG & 78.89 & 64.69 & 47.52 & 29.05 & 12.53 & 3.47 & 0.56 & 0.13\\
Attn-HG & 76.48 & 59.27 & 39.71 & 20.34 & 7.49 & 2.09 & 0.46 & 0.21\\
DLCM & 77.07 & 61.59 & 41.97 & 22.56 & 7.42 & 1.75 & 0.47 & 0.19\\
\hline
\end{tabular}
\vspace{0.3em}
\caption{\textbf{Relative PCKh} results for different $\epsilon$ values for \textbf{IGSM-U-100} attacks on all model}
\label{table:UI_100}
\end{table*}

\begin{table*}
\centering
\begin{tabular}{c c c c c c c c c}
\hline
Model & 0.25 & 0.5 & 1 & 2 & 4 & 8 & 16 & 32\\[0.5ex]
\hline
DeepPose & 8.33 & 15.77 & 39.78 & 80.27 & 97.84 & 98.97 & 99.06 & 98.85\\
Chained & 5.84 & 11.14 & 26.41 & 60.48 & 90.53 & 97.76 & 98.9 & 99.18\\
2-SHG & 6.12 & 15.7 & 39.24 & 63.84 & 76.58 & 82.96 & 86.52 & 88.43\\
8-SHG & 5.93 & 13.0 & 34.33 & 66.62 & 86.63 & 94.07 & 96.47 & 97.52\\
Attn-HG & 7.82 & 19.39 & 42.7 & 66.95 & 80.73 & 86.79 & 90.37 & 92.76\\
DLCM & 7.67 & 15.65 & 34.08 & 95.41 & 82.21 & 91.38 & 94.69 & 95.98\\
\hline
\end{tabular}
\vspace{0.3em}
\caption{\textbf{Absolute PCKh} with respect to the target results for different $\epsilon$ values for \textbf{IGSM-T-100} attacks on all model}
\label{table:TI_100}
\end{table*}

\begin{table*}[!h]
\begin{center}
 \begin{tabular}{c c c c c c c c c}
 \hline
 & newell & newell- & attention & DLCM & 2-SHG- & 2-SHG & chain- & Deep- \\ [0.5ex]
 & newell & all & attention & DLCM & all & 2HG & pred & Pose \\ [0.5ex]
 \hline

 newell &26.25 &31.75 &81.56 &77.29 &53.45 &68.17 &63.23 &86.7 \\
%  \hline
 attention &70.65 &69.99 &31.15 &79.27 &61.05 &71.68 &68.1 &84.78 \\
%  \hline
 DLCM &80.46 &79.23 &87.18 &39.41 &64.45 &74.02 &67.41 &84.93 \\
%  \hline
 2HG &72.67 &72.15 &86.18 &83.21 &28.09 &46.14 &81.34 &96.42 \\
%  \hline
 chain-pred &89.01 &87.97 &92.42 &91.34 &88.56 &92.51 &52.89 &91.85 \\
%  \hline
 DeepPose &81.71 &79.75 &87.06 &83.51 &82.81 &87.3 &68.65 &27.85 \\
%  \hline
 \end{tabular}
\end{center}
\caption{Results of all source-target pairs under the doubly black box setting of universal perturbations for an $\epsilon$ value of 8}
\label{table:univ_bb_8}
 \end{table*}

\begin{table*}[!h]
\centering
\begin{tabular}{c c c c c c c c c}
\hline
Model & 0.25 & 0.5 & 1 & 2 & 4 & 8 & 16 & 32\\[0.5ex]
\hline
Chained & 81.74 & 69.25 & 52.36 & 33.37 & 16.59 & 7.38 & 3.17 & 1.54\\
2-SHG & 80.59 & 69.67 & 56.4 & 41.69 & 27.0 & 15.2 & 7.27 & 2.95\\
DeepPose & 91.25 & 79.4 & 57.82 & 31.13 & 11.11 & 3.31 & 1.2 & 0.49\\
\hline
\end{tabular}
\vspace{0.3em}
\caption{\textbf{Relative PCK} on the COCO dataset results for different $\epsilon$ values under \textbf{IGSM-U-10} attacks on all models}
\label{table:COCO_UI}
\end{table*}

%----------------------------------------------------------------------------
\begin{table*}[!h]
\centering
\begin{tabular}{c c c c c c c c c}
\hline
Model & 0.25 & 0.5 & 1 & 2 & 4 & 8 & 16 & 32\\[0.5ex]
\hline
Chained & 4.76 & 8.33 & 15.55 & 28.23 & 44.69 & 58.62 & 65.89 & 67.49\\
2-SHG & 5.59 & 10.87 & 22.25 & 41.62 & 61.78 & 73.9 & 79.21 & 79.78\\
DeepPose & 3.3 & 4.86 & 7.99 & 12.98 & 18.26 & 21.33 & 22.79 & 23.12\\
\hline
\end{tabular}
\vspace{0.3em}
\caption{Absolute PCK on the COCO dataset with respect to the target labels for different $\epsilon$ values under IGSM-T-20 attacks on all models}
\label{table:COCO_TI}
\end{table*}

%----------------------------------------------------------------------------
\begin{table*}[!h]
\centering
\begin{tabular}{c c c c c c c c c}
\hline
Model & 0.25 & 0.5 & 1 & 2 & 4 & 8 & 16 & 32\\[0.5ex]
\hline
Chained & 87.61 & 81.68 & 75.34 & 69.17 & 63.96 & 60.49 & 58.63 & 50.67\\
2-SHG & 87.51 & 82.31 & 77.01 & 72.47 & 69.2 & 67.03 & 63.7 & 48.21\\
DeepPose & 94.54 & 89.5 & 82.72 & 74.9 & 67.93 & 63.48 & 61.45 & 48.67\\
\hline
\end{tabular}
\vspace{0.3em}
\caption{Relative PCK on the COCO dataset for different $\epsilon$ values under FGSM-U attacks on all models}
\label{table:COCO_UF}
\end{table*}

%----------------------------------------------------------------------------
\begin{table*}[!h]

\centering

\begin{tabular}{c c c c c c c c c}
\hline
Model & 0.25 & 0.5 & 1 & 2 & 4 & 8 & 16 & 32\\[0.5ex]
\hline
Chained & 3.41 & 4.13 & 4.86 & 5.5 & 6.06 & 6.31 & 6.26 & 5.14\\
2-SHG & 3.37 & 3.98 & 4.69 & 5.22 & 5.74 & 5.95 & 5.94 & 6.47\\
DeepPose & 2.89 & 3.36 & 4.0 & 4.54 & 4.92 & 5.18 & 5.36 & 5.96\\
\hline
\end{tabular}
\vspace{0.3em}
\caption{Absolute PCK on the COCO dataset with respect to the target labels for different $\epsilon$ values under FGSM-T attacks on all models}
\label{table:COCO_TF}
\end{table*}

\begin{table*}
\centering
 \begin{tabular}{c c c c c c c c c c}
\hline

Model &Nose &Eye &Ear &Shoulder &Elbow &Wrist &Hip &Knee &Ankle \\[0.5ex]
\hline \hline
& \multicolumn{6}{c}{\textbf{Relative PCKh}} \\
\hline
DeepPose & 7.89 & 5.97 & 3.65 & 4.71 & 1.70 & 2.10 & 0.95 & 0.26 & 0.24 \\
2-SHG & 29.02 & 33.37 & 32.30 & 20.46 & 5.79 & 4.19 & 3.62 & 2.97 & 2.15 \\
Chained & 11.25 & 11.10 & 16.63 &  11.95 & 3.34 &  2.19 & 3.26 &  1.89 & 1.61 \\

\hline 
\end{tabular}
\vspace{0.3em}
\caption{Relative PCKh of different body-joints for untargeted attacks across different models on the COCO dataset. Note that hips, knee and ankles are more vulnerable than the rest.}
\label{table:COCO_joints}
\end{table*}

\begin{table*}[!h]
\begin{center}
\begin{tabular}{l|c}
\hline
Model & PCK on Validation Set \\
\hline
2-SHG & 85.0\\
Chained & 81.4\\
DeepPose & 70.4\\
\hline
\end{tabular}
\end{center}
\caption{Table showing the original performance of the models on the validation set (for the COCO Keypoints dataset) under our experimental setup}
\label{table:COCO_original}
\end{table*}
\vspace{-10pt}

\begin{table*}[!h]
\begin{center}
\begin{tabular}{l| c|  c | c }
\hline
Model & Raw Attacks & Flipping & Gaussian Blurring\\[0.5ex]
\hline

8-SHG & 20.4 & 69.61 & 68.90\\
Attn-HG & 31.14 & 82.85 & 75.39\\
DLCM & 39.41 & 71.14 & 68.89\\
2-SHG & 15.18 & 64.3 & 62.7\\
Chained & 7.6 & 67.15 & 73.3\\
DeepPose & 5.6 & 56.9 & 47.6\\

\end{tabular}
\end{center}
\caption{Effectiveness of flipping and gaussian blurring on image dependent (IGSM-U-10) attacks (MPII dataset)}
\label{table:untarDefense}
\end{table*}

\begin{table*}[!h]
\begin{center}
\begin{tabular}{l | c |  c |  c}
\hline
Model & Raw Attacks & Flipping & Gaussian Blurring\\[0.5ex]
\hline

8-SHG & 8.85 & 25.82 & 43.24\\ 
Attn-HG & 11.47 & 56.24 & 57.05\\
DLCM & 12.75 & 44.02 & 52.36\\
2-SHG & 13.8 & 13.8 & 59.3\\
Chained & 9.0 & 9.0 & 45.5\\
DeepPose & 1.6 & 1.5 & 28.4\\

\end{tabular}
\end{center}
\caption{Effectiveness of flipping and gaussian blurring on universal adversarial perturbations (MPII dataset)}
\label{table:universalDefense}
\end{table*}

%----------------------------------------------------------------------------
%----------------------------------------------------------------------------
\vspace{-20em}
\begingroup
\raggedright
